# Supplementary material for: Is there a background population of high-albedo objects in geosynchronous orbits around Earth?
Source: arXiv:2204.06091 source file (2022-04-12)
Supplement: Supplementary file 1 [file Appendix.pdf]

# Appendix

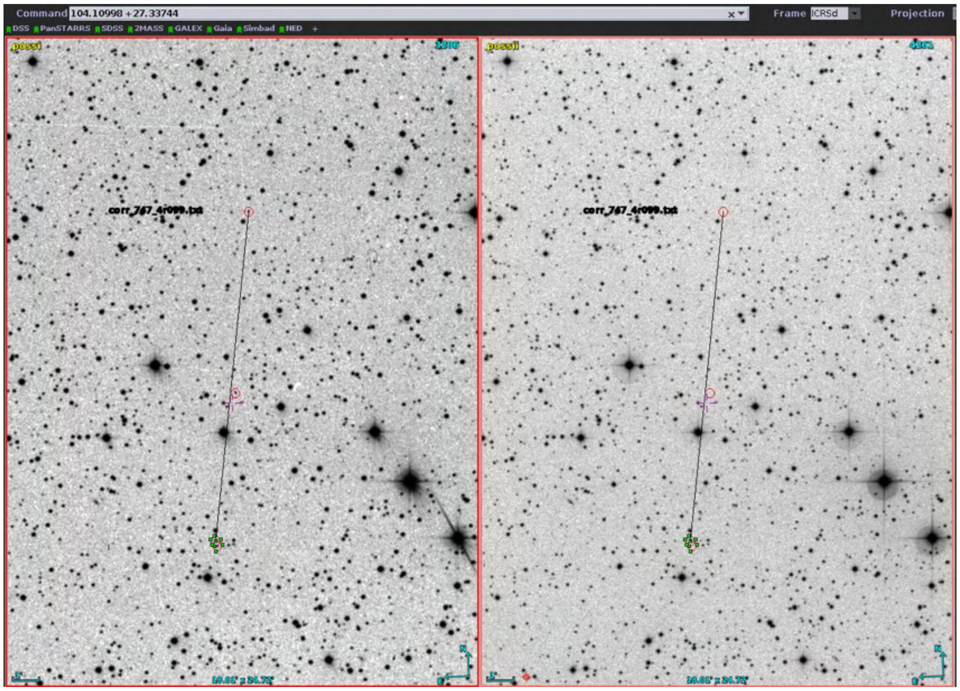


Figure 1

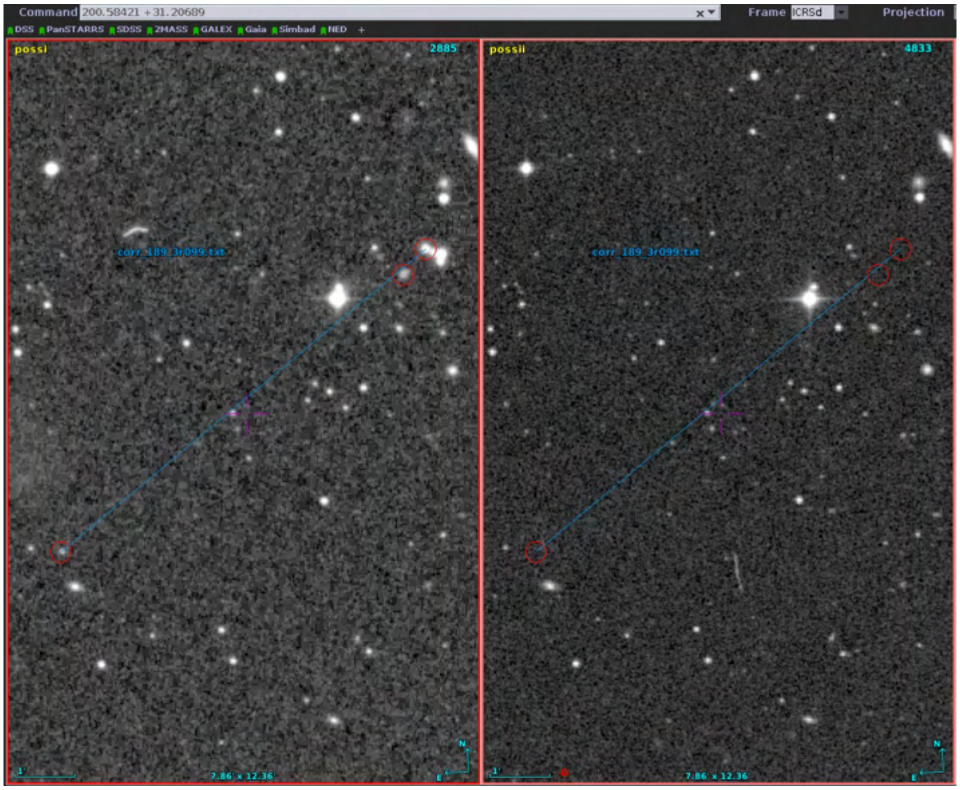


Figure 2

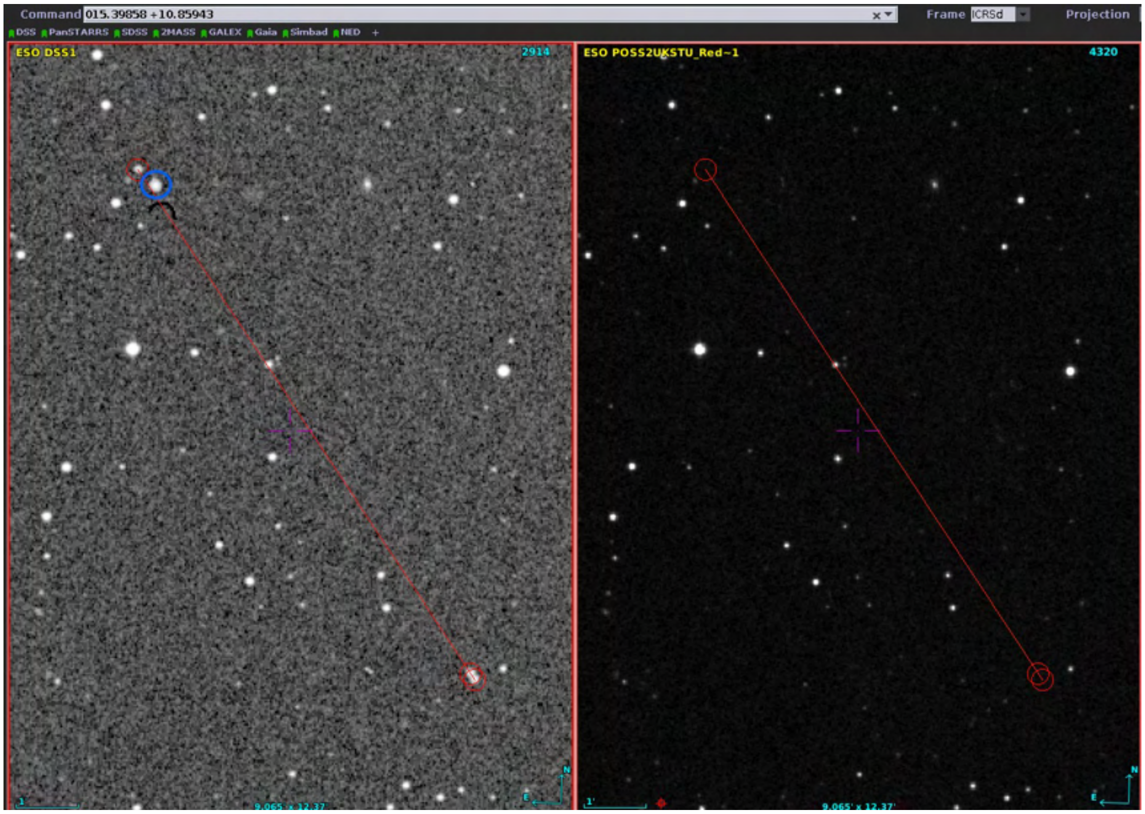


**Figure 3**

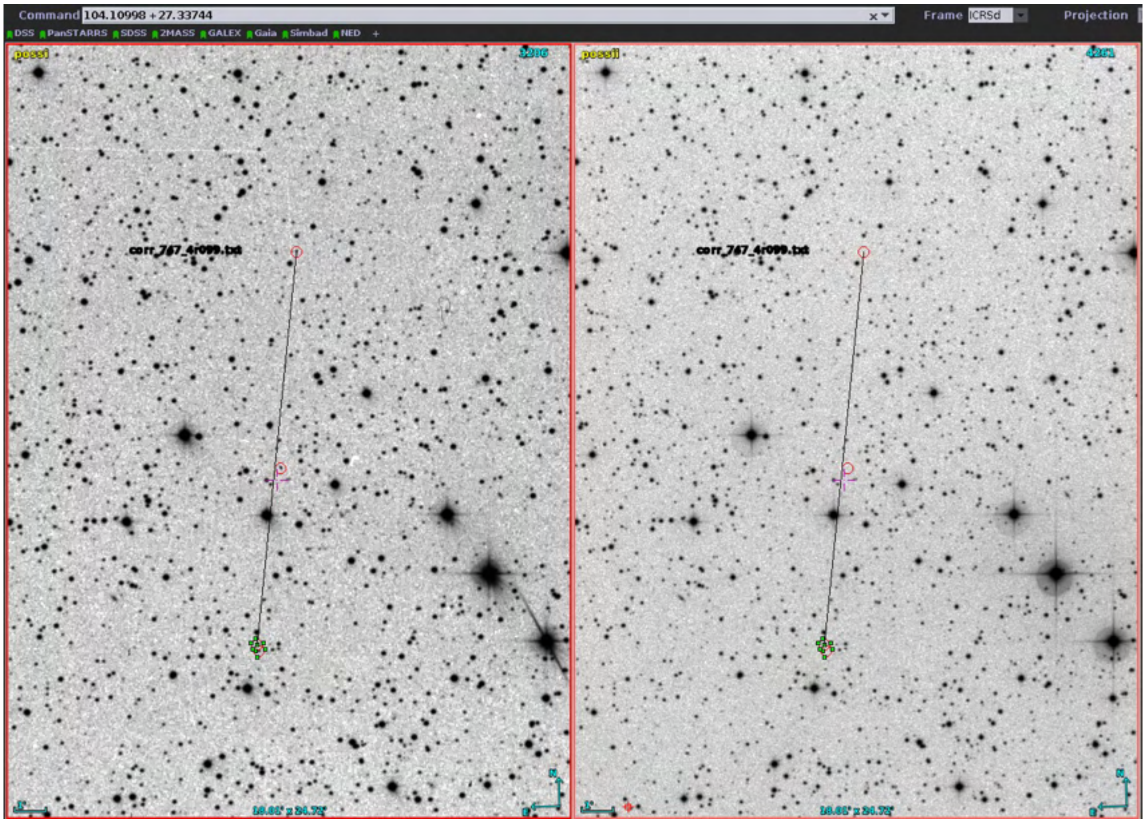


**Figure 4**

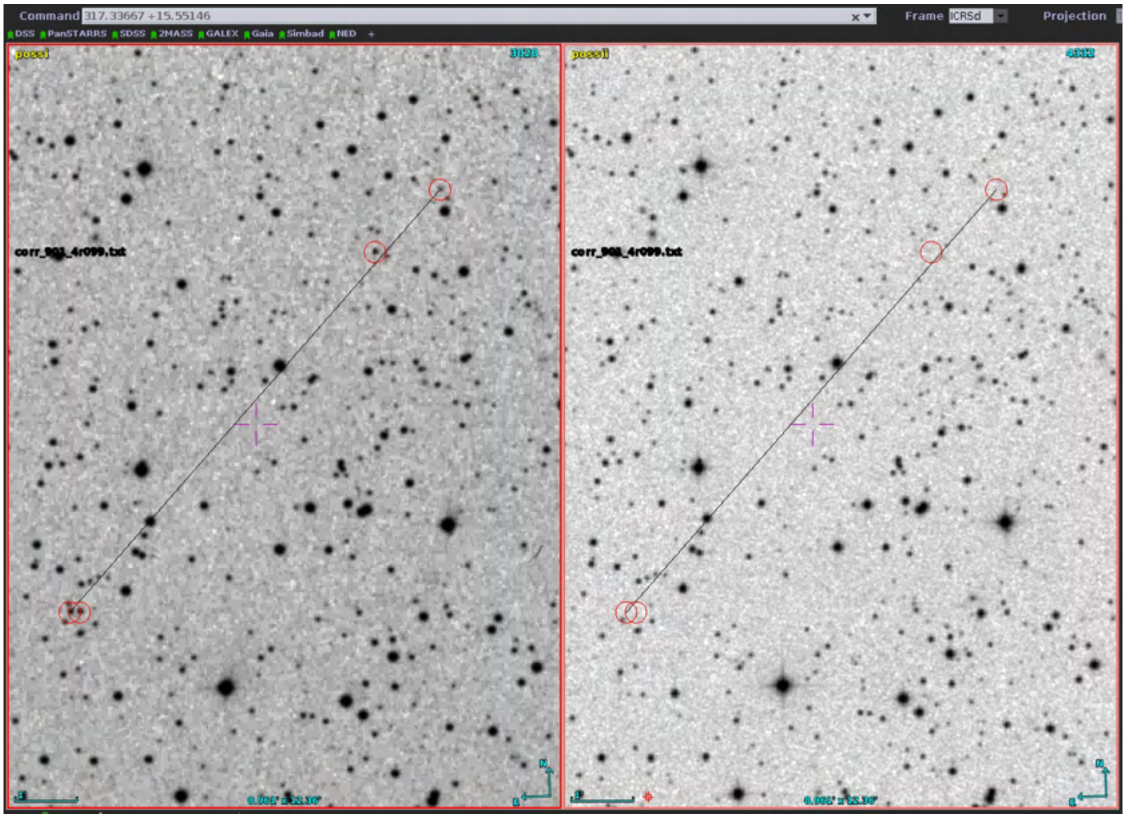


**Figure 5**

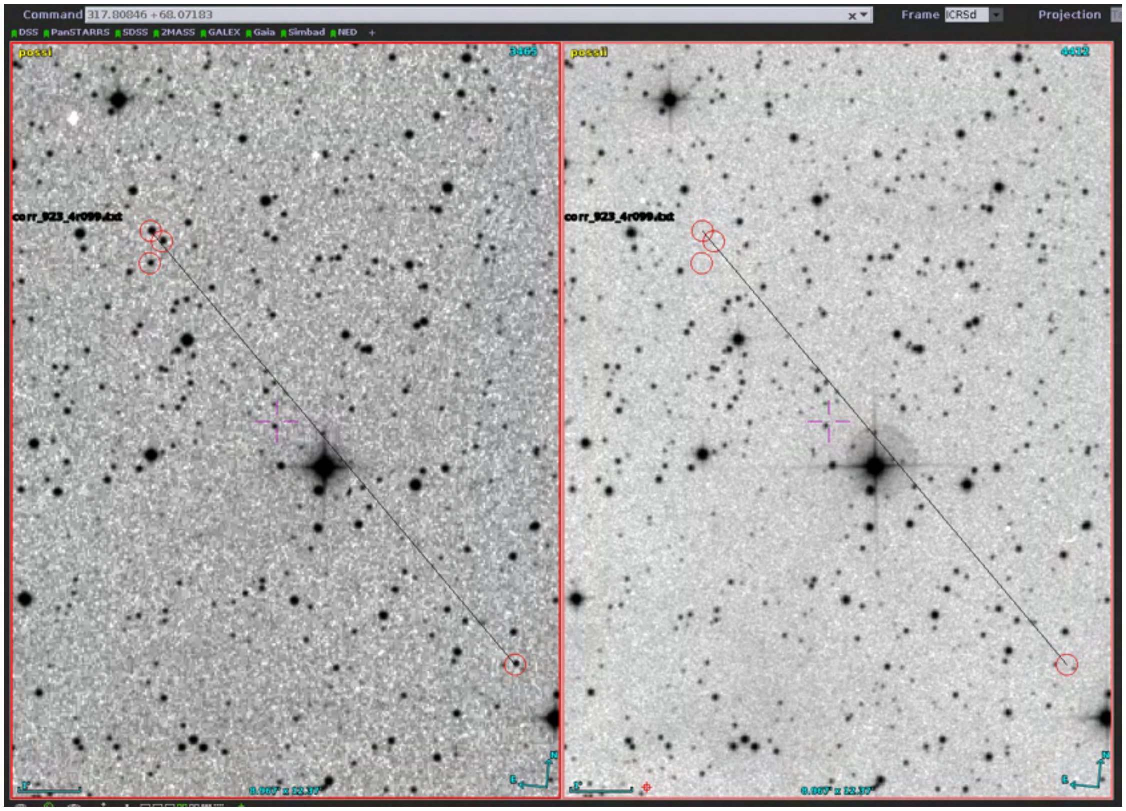


**Figure 6**

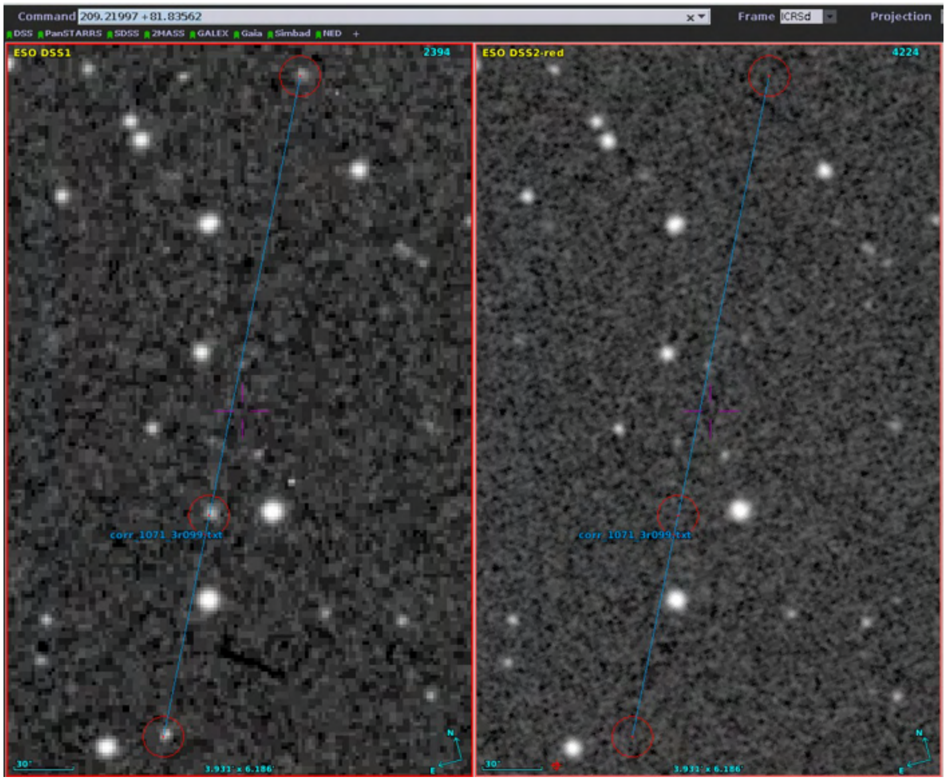


Figure 7

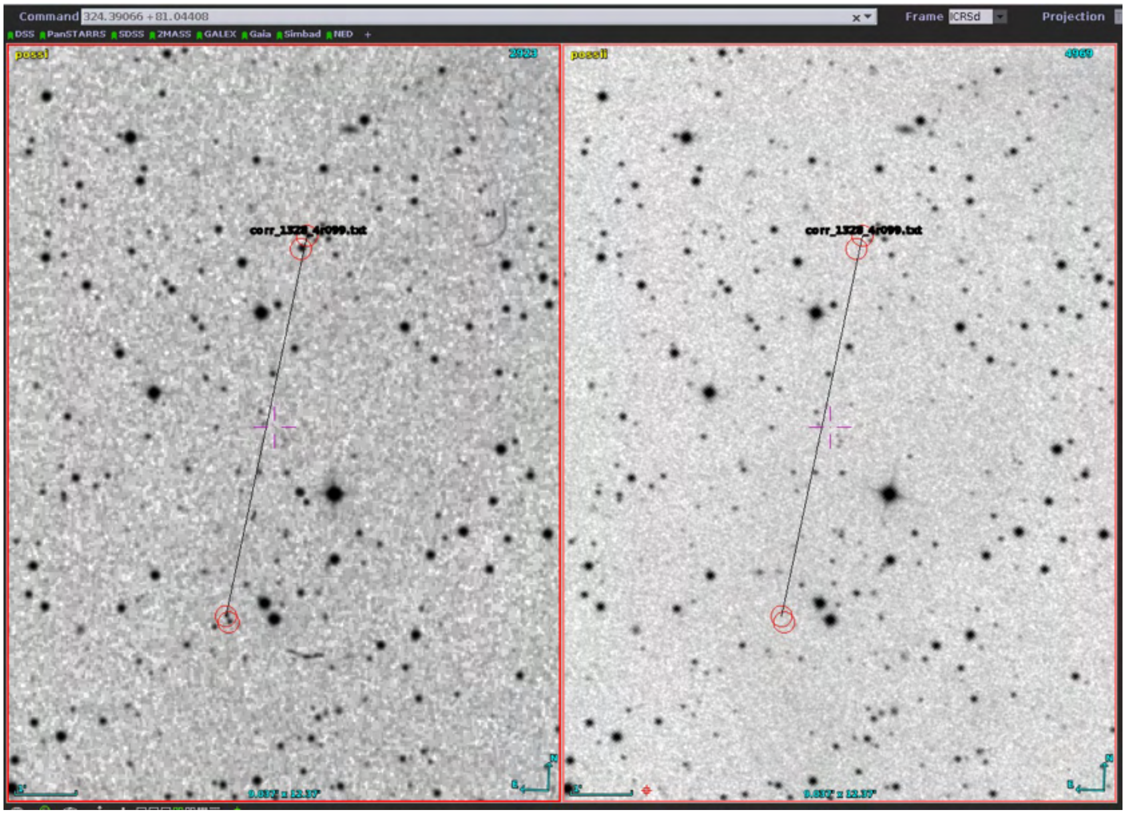


Figure 8

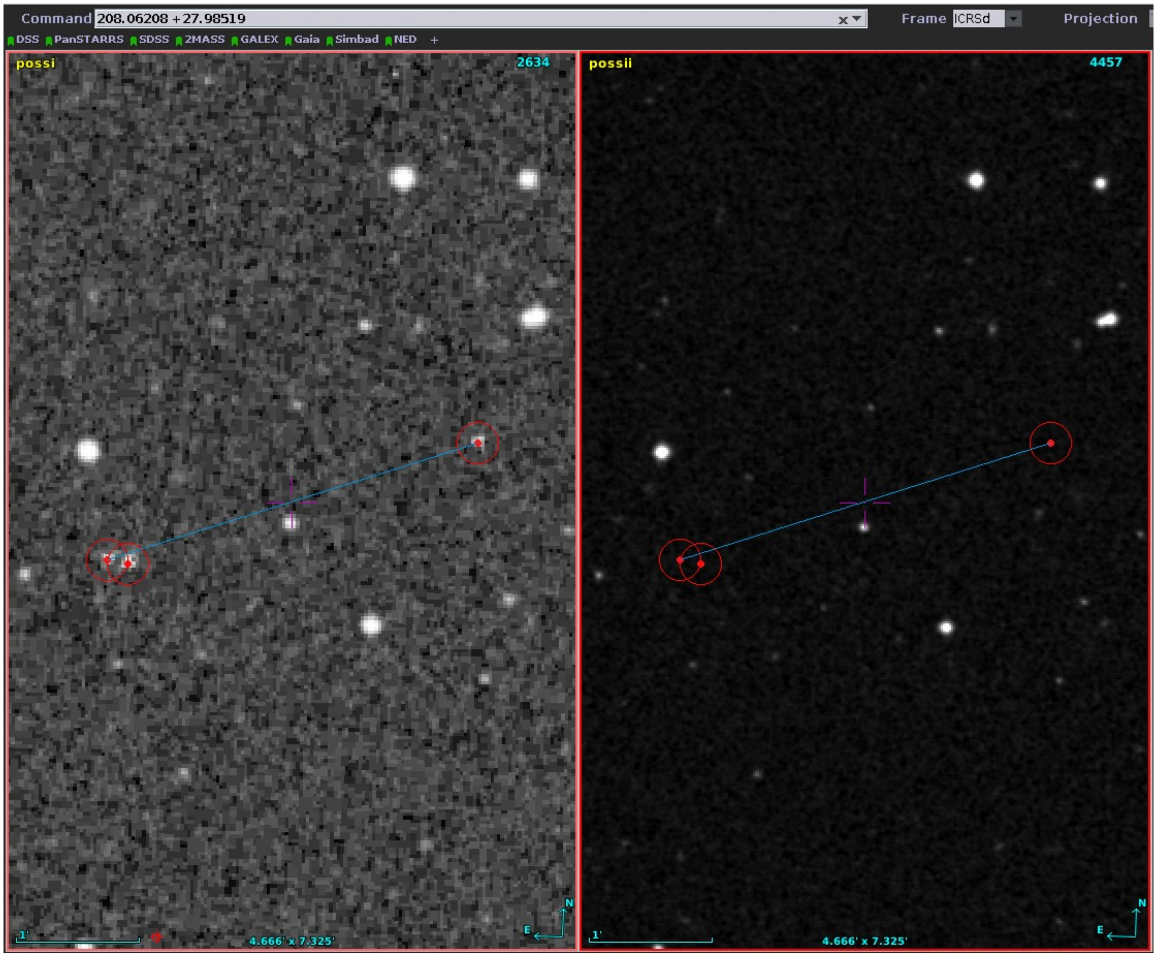


Figure 9

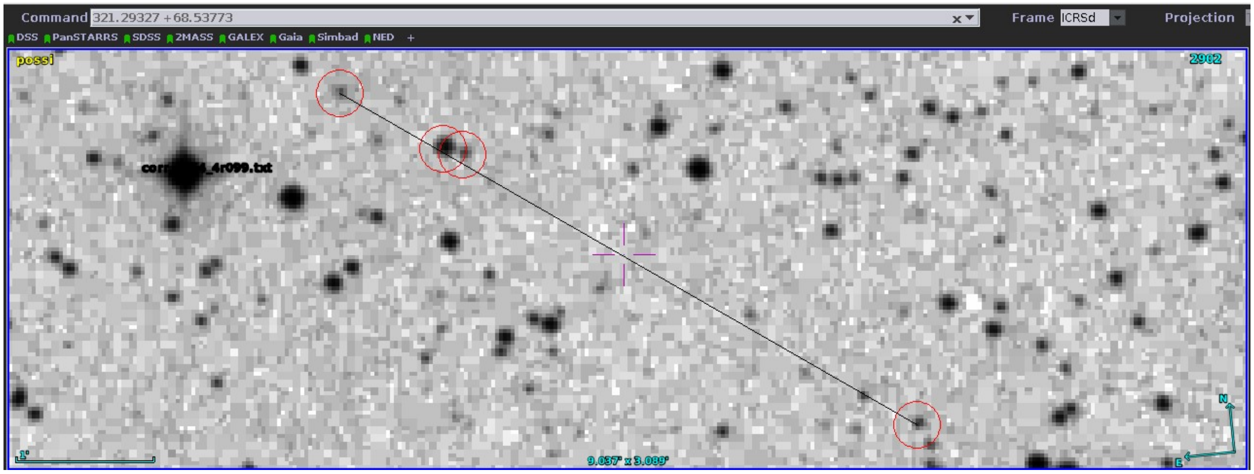


Figure 10

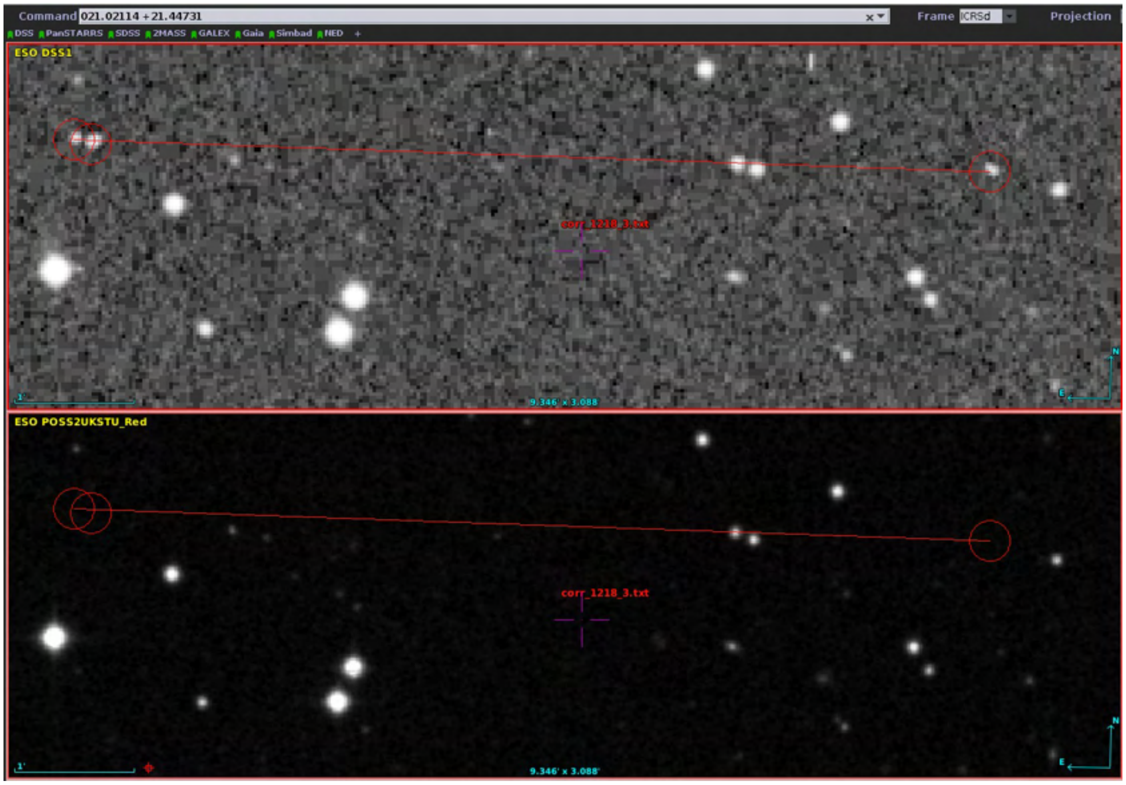


**Figure 11**

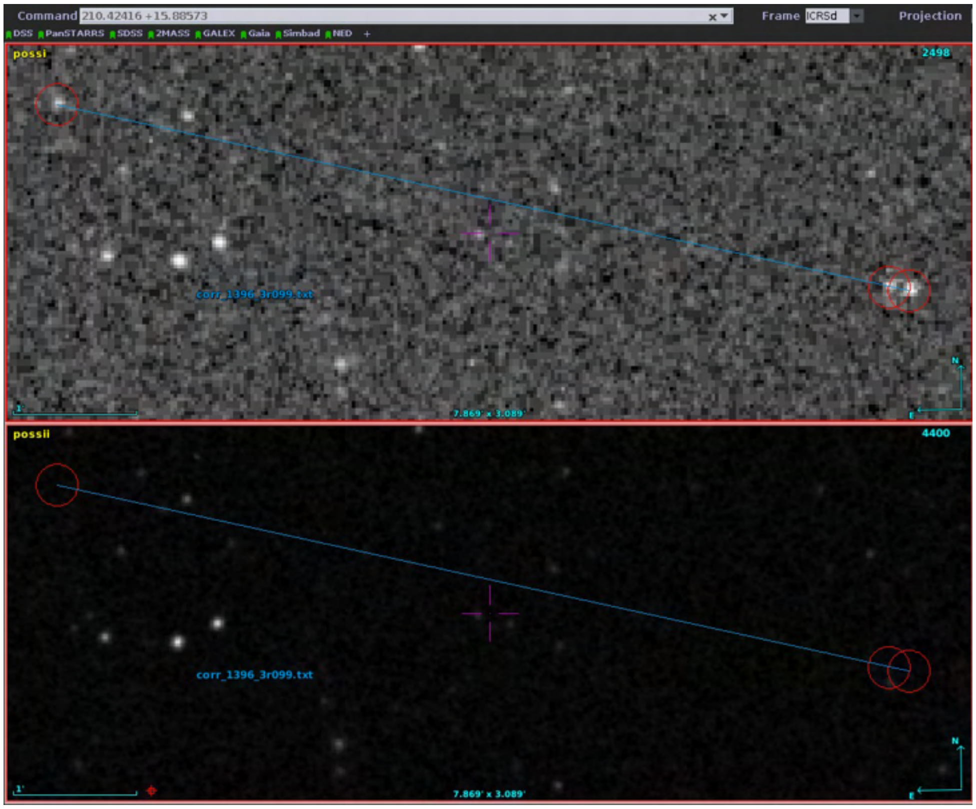


**Figure 12**

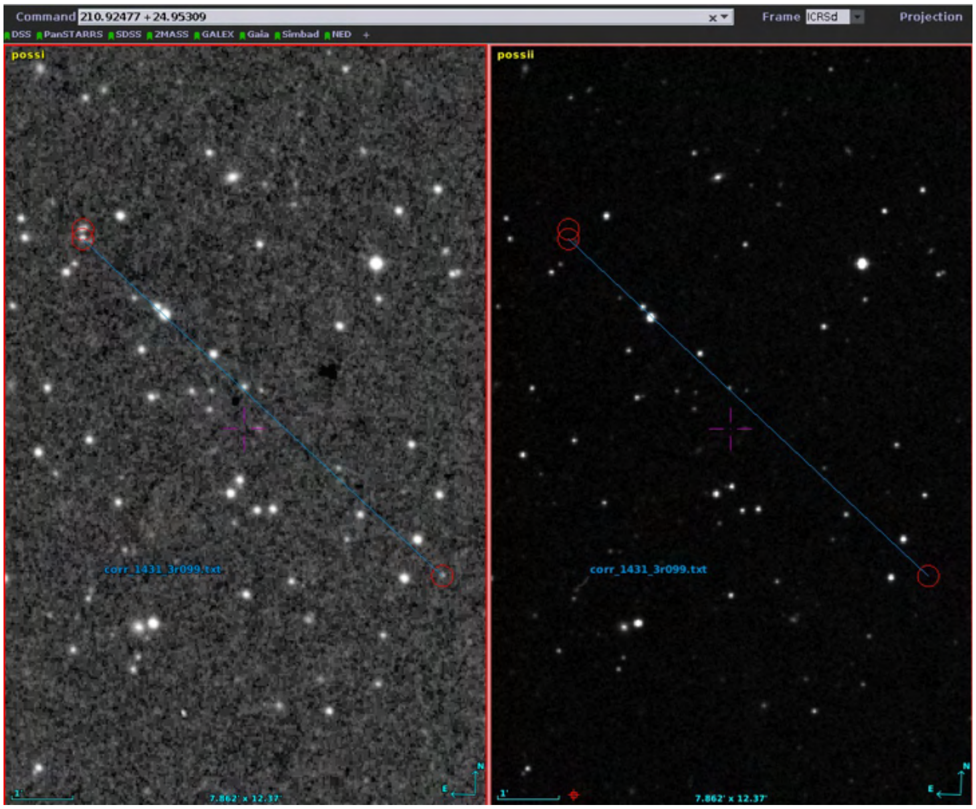


# Figure 13

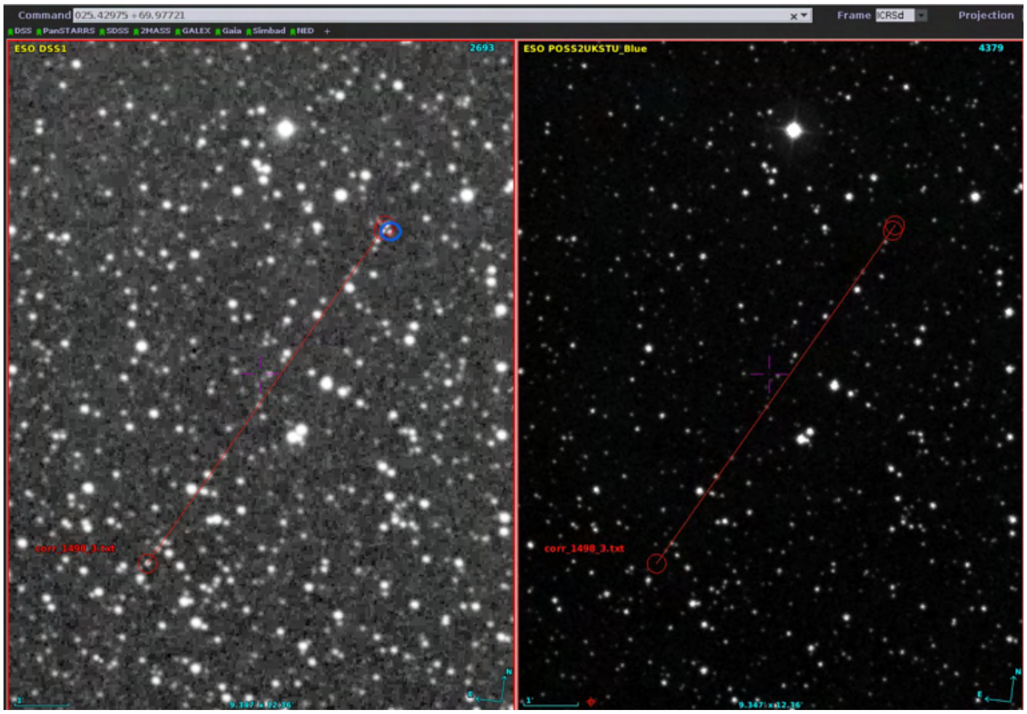


# Figure 14

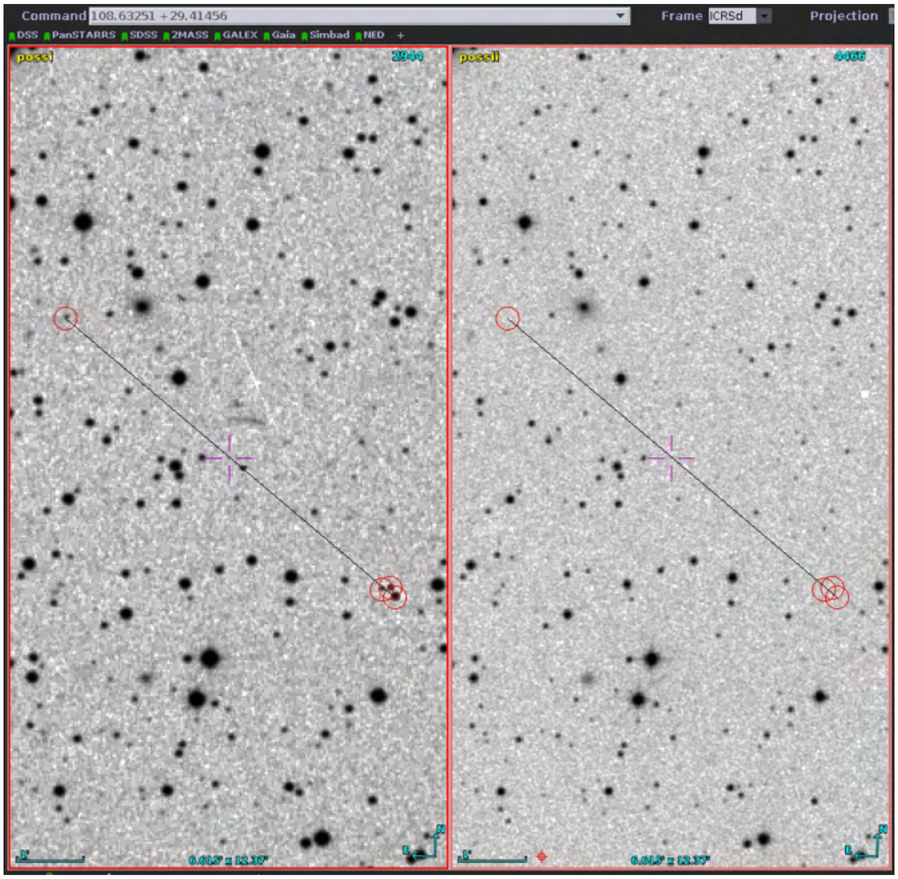


Figure 15

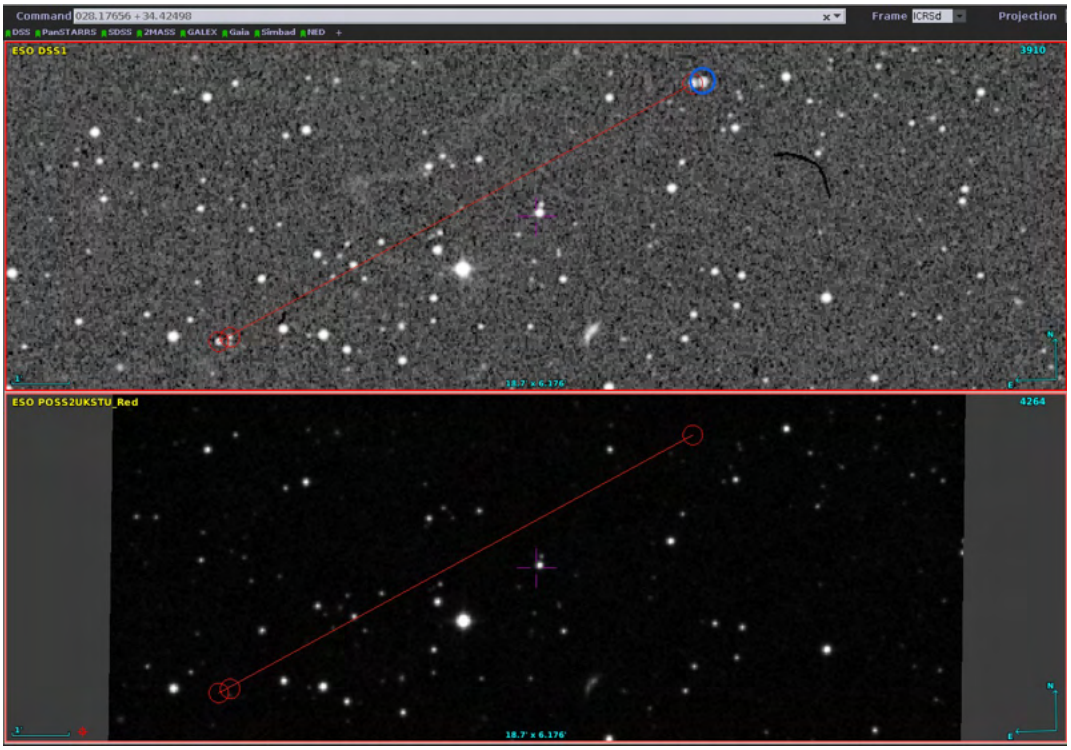


Figure 16

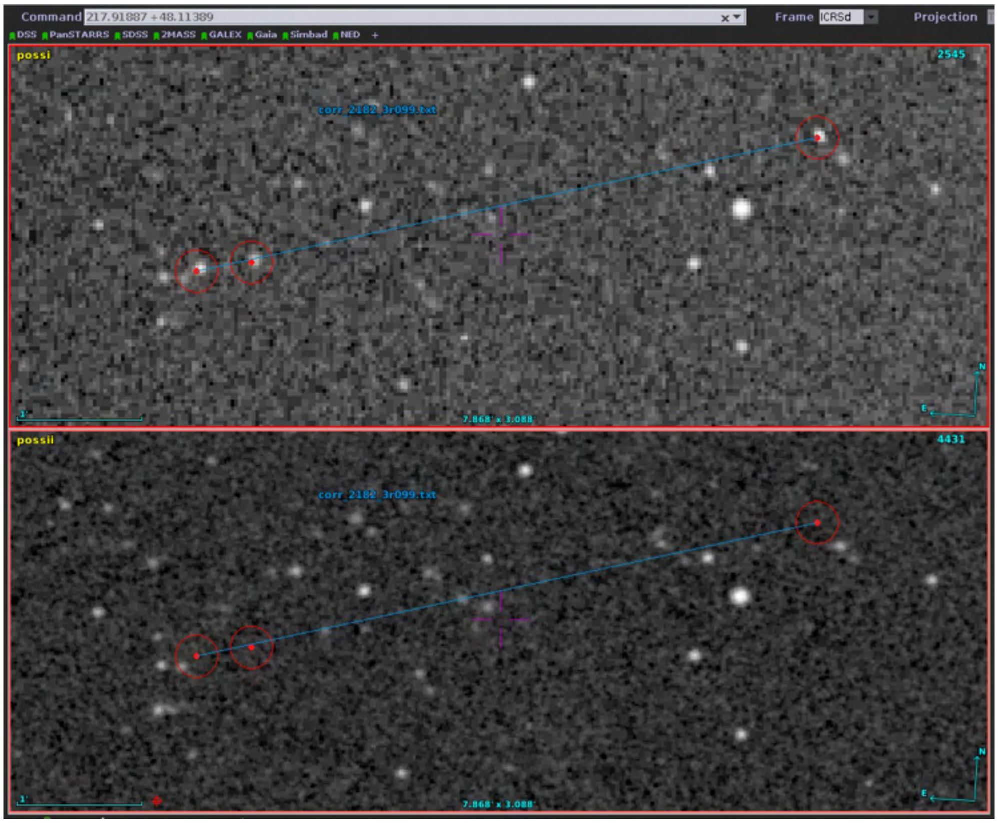


Figure 17

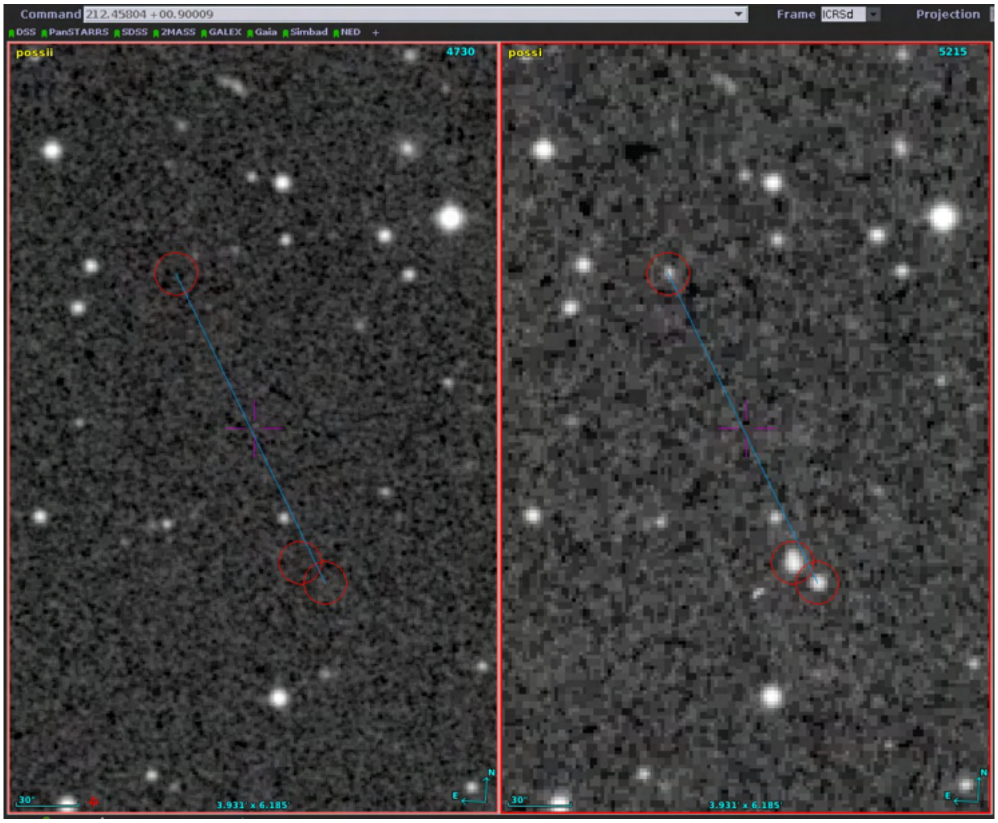


Figure 18

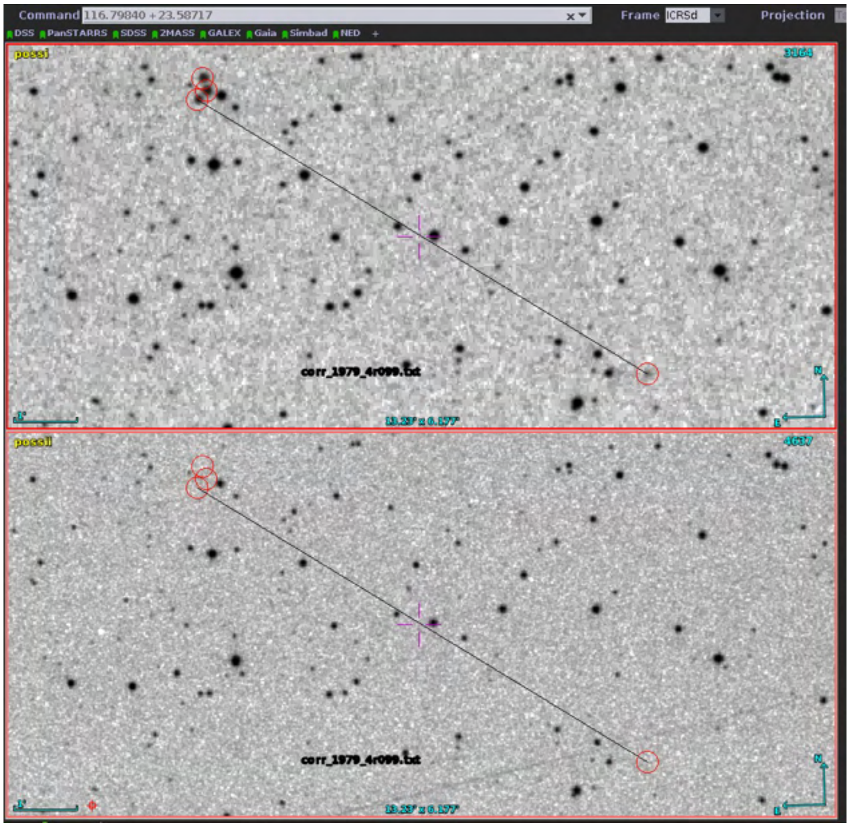


Figure 19

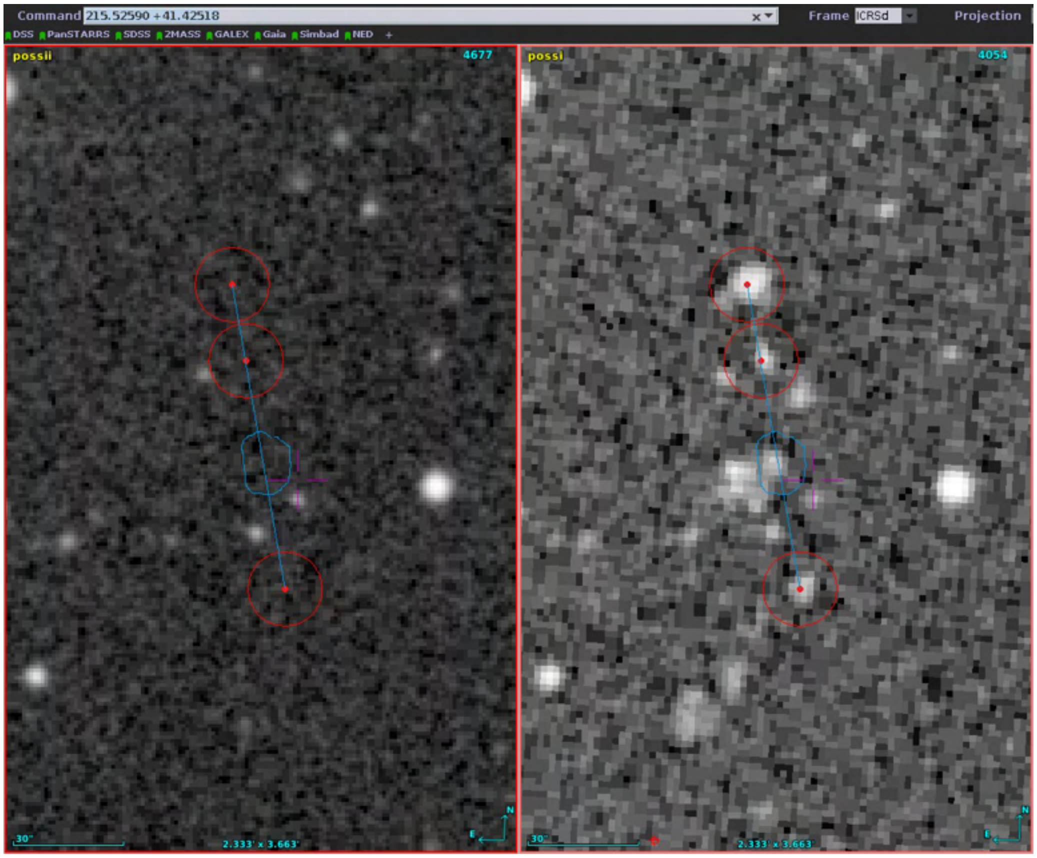


Figure 20

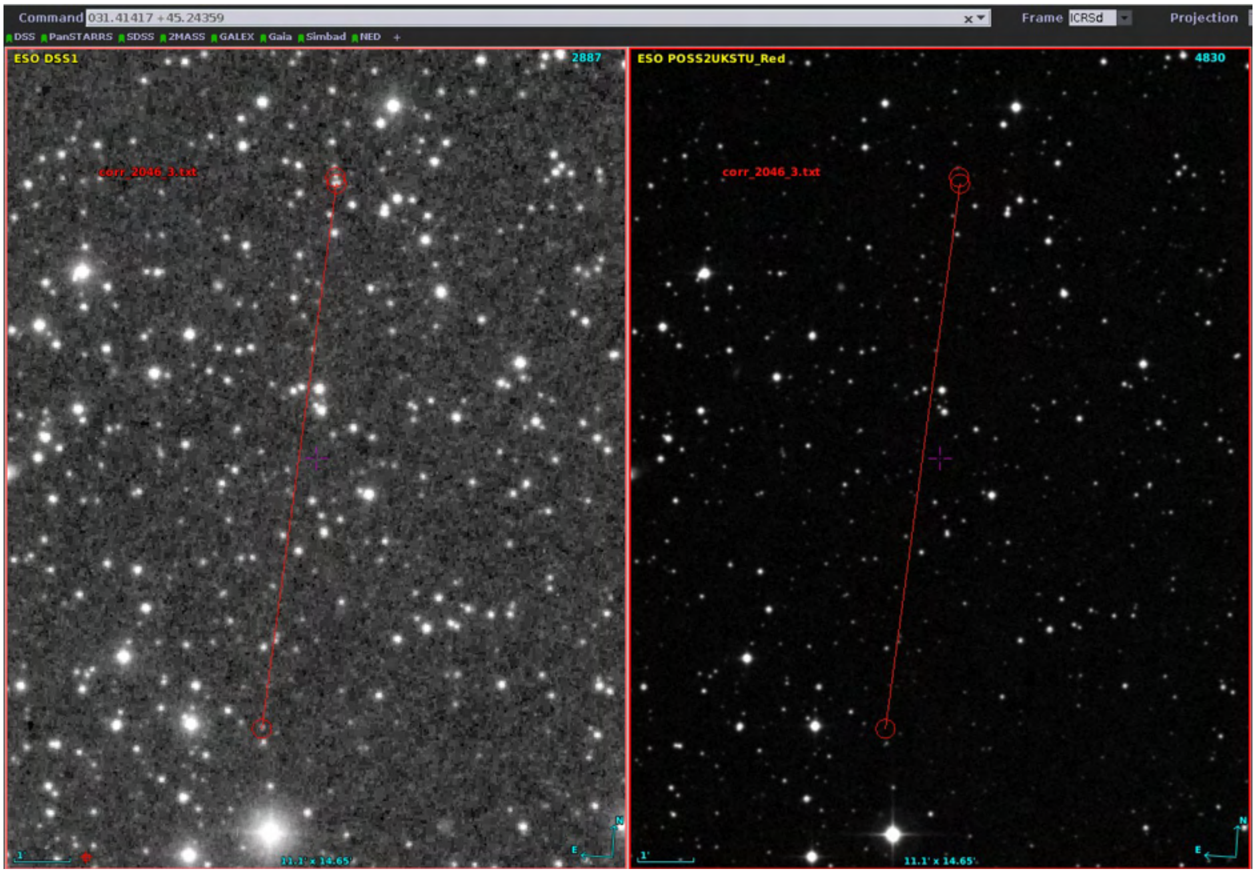


Figure 21

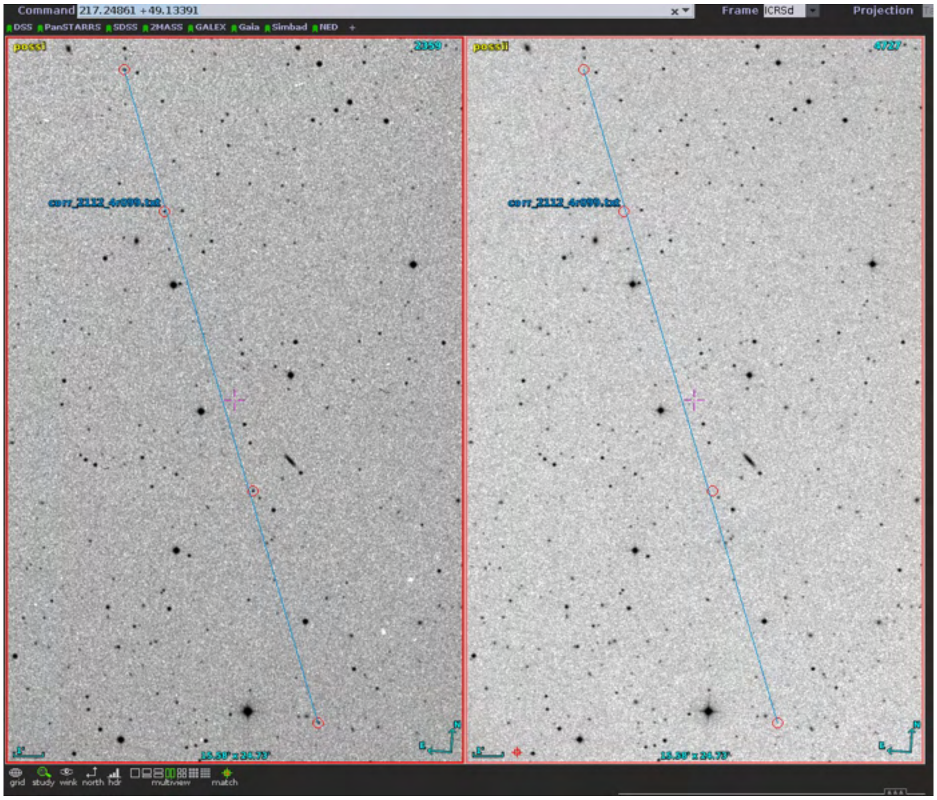


Figure 22

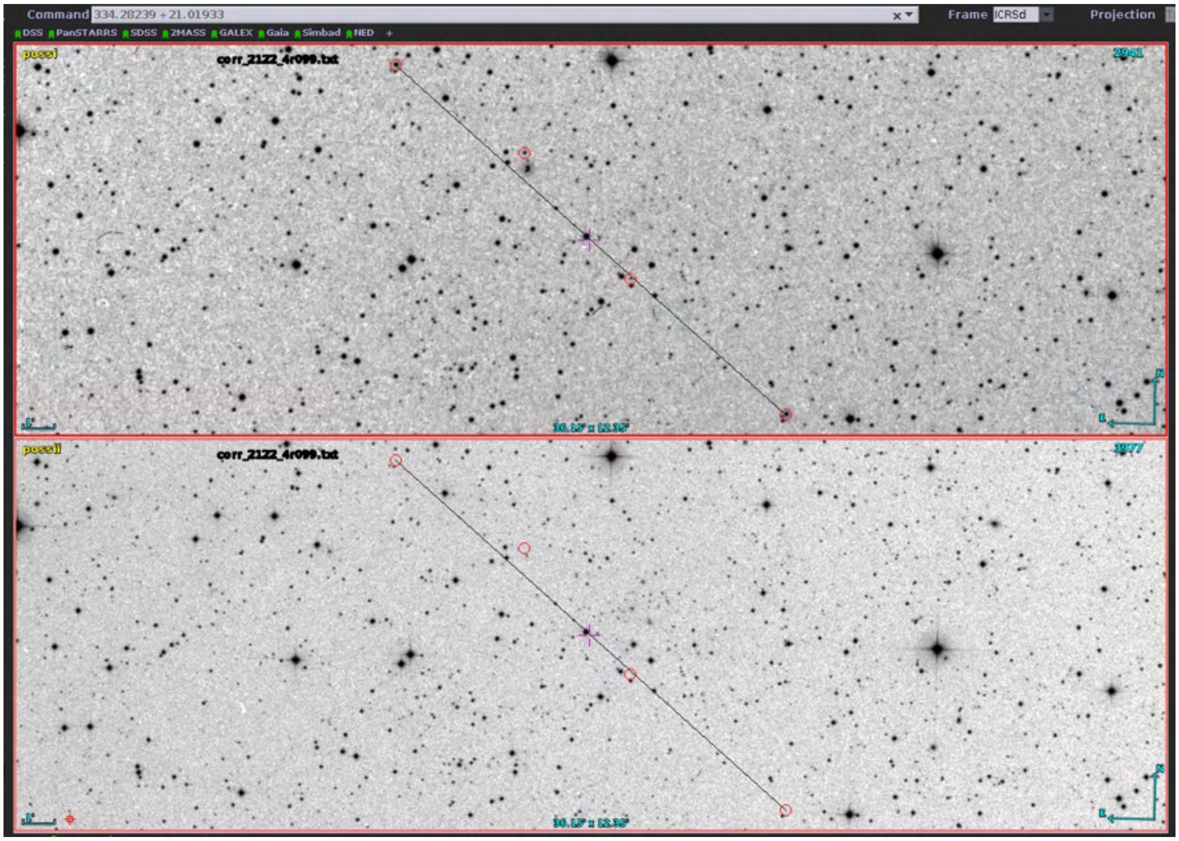


**Figure 23**

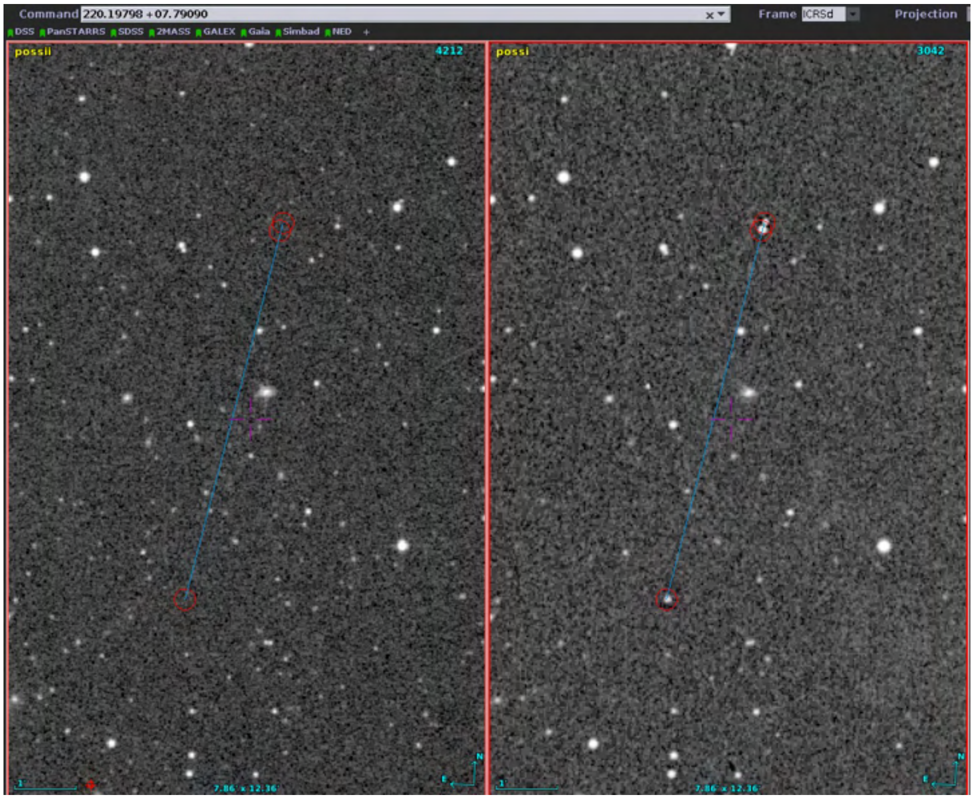


**Figure 24**

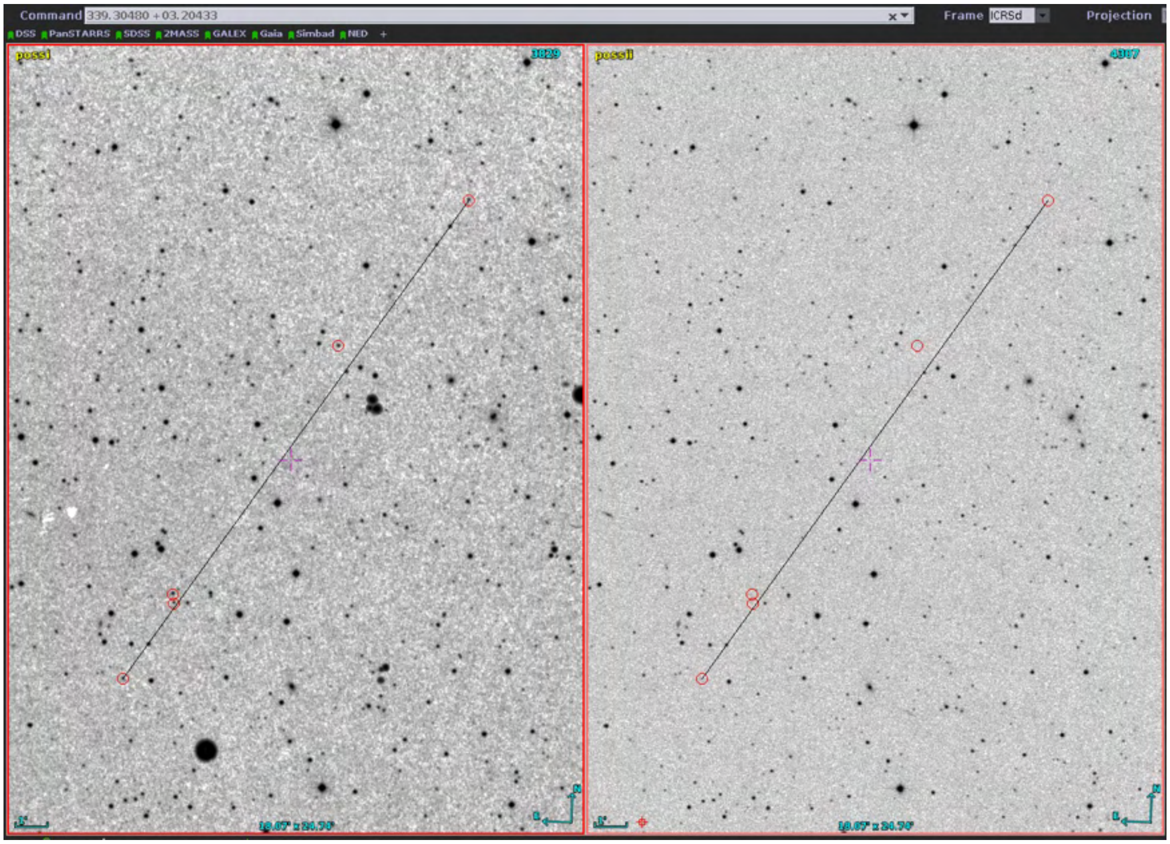


Figure 25

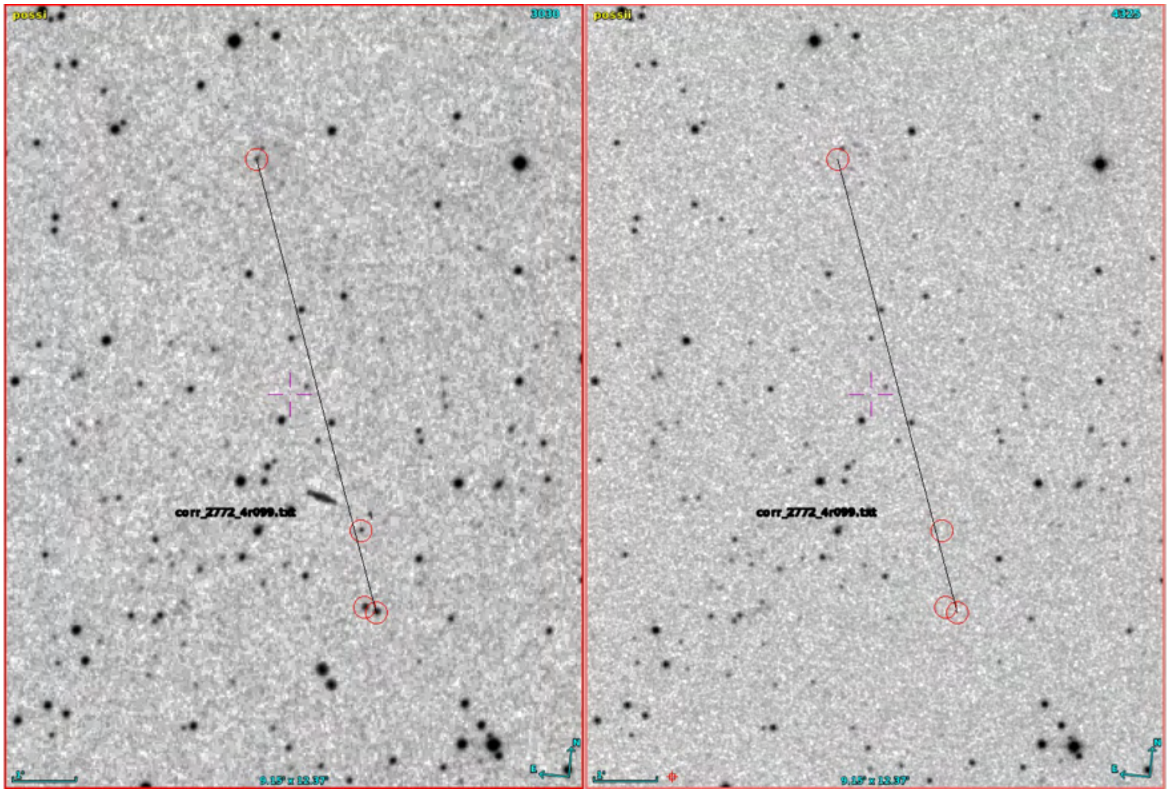


Figure 26

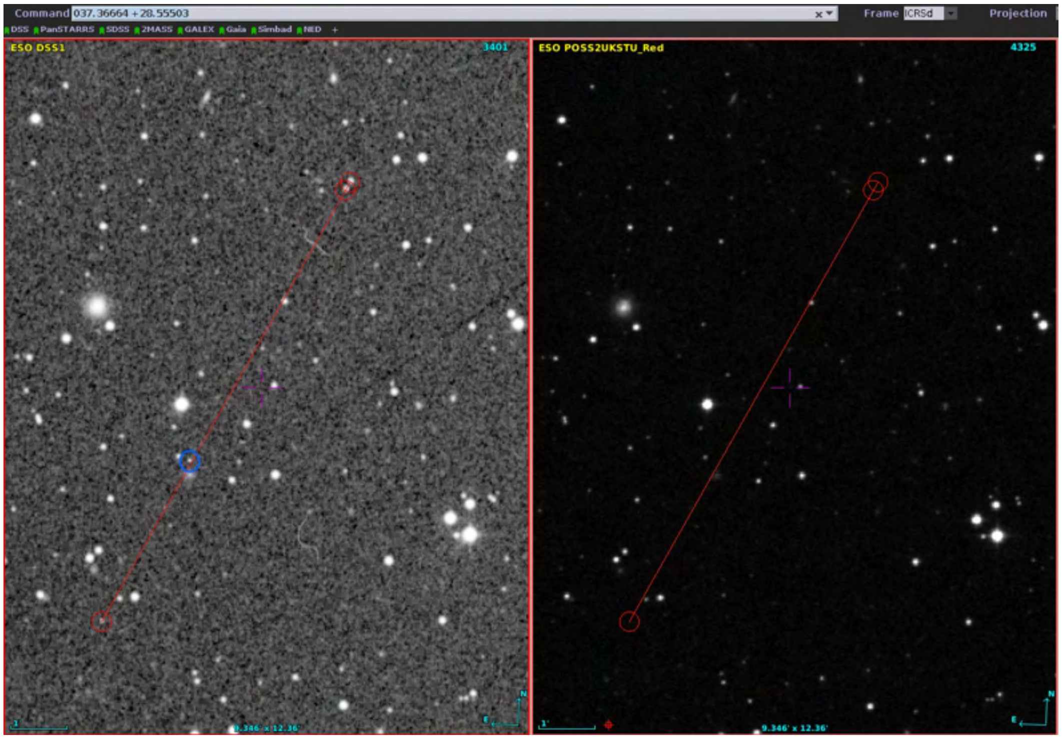


Figure 27

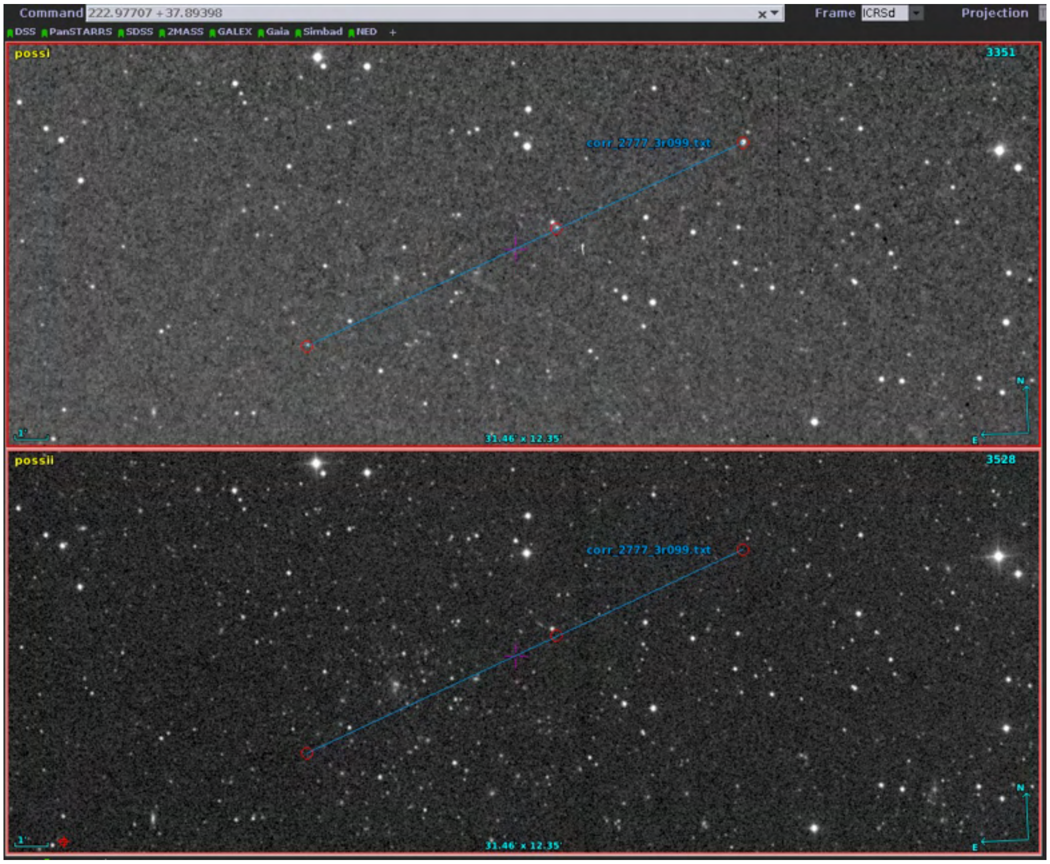


Figure 28

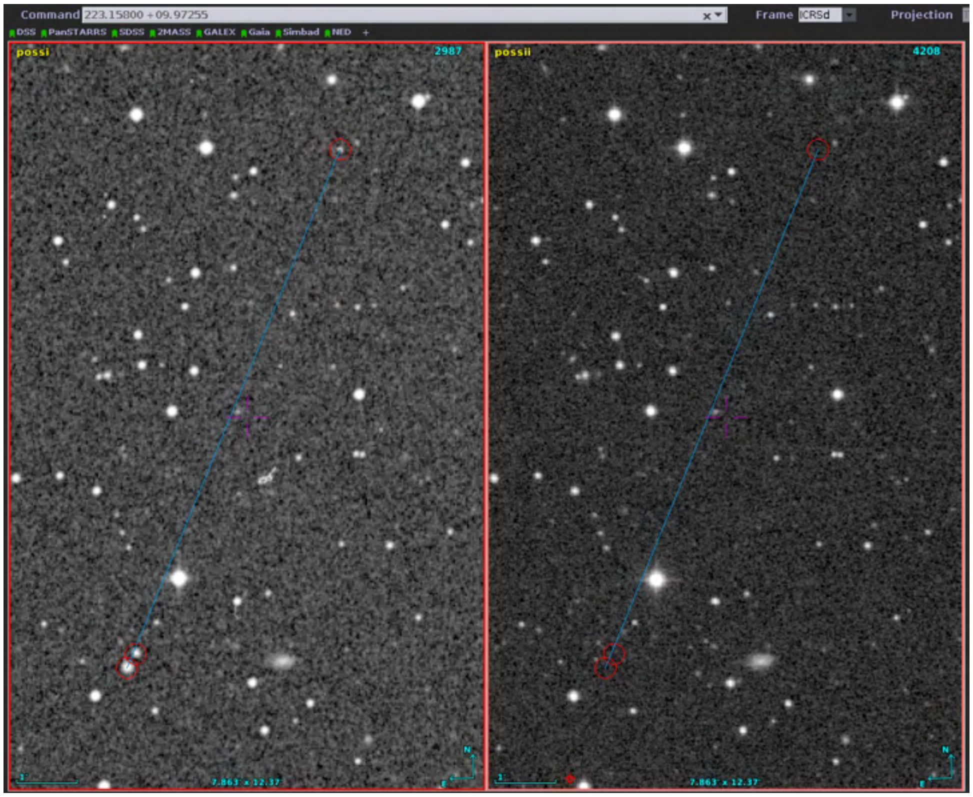


# Figure 29

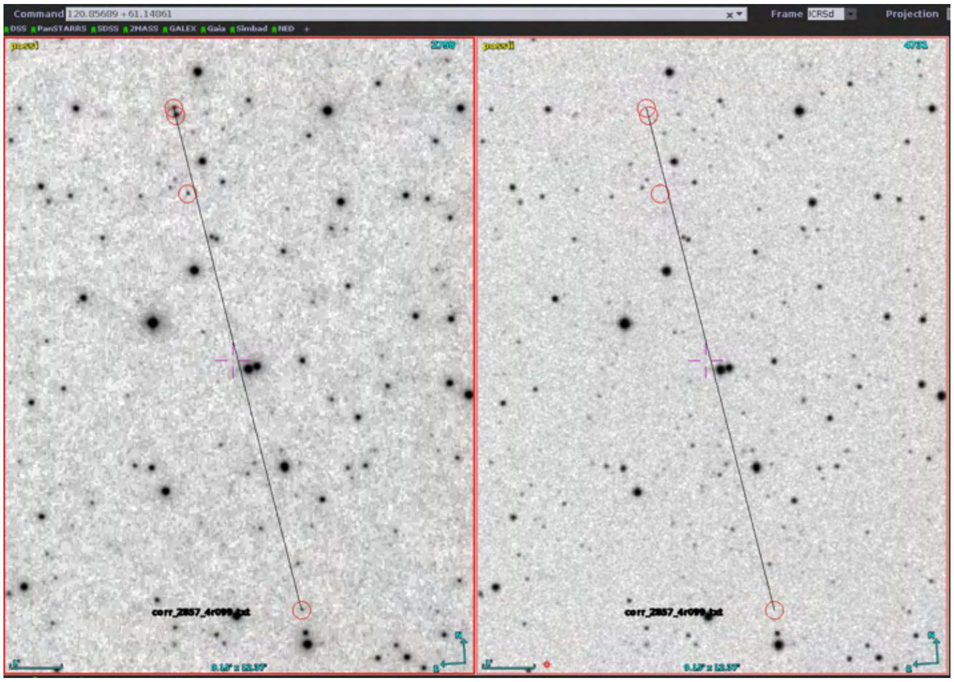


# Figure 30

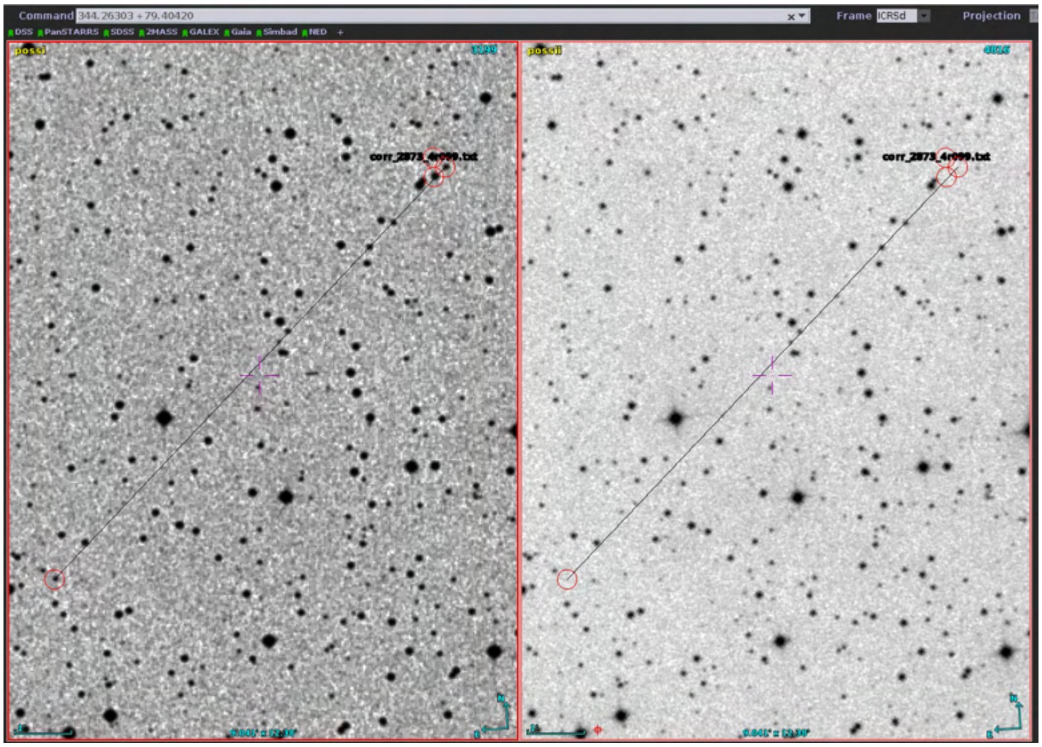


**Figure 31**

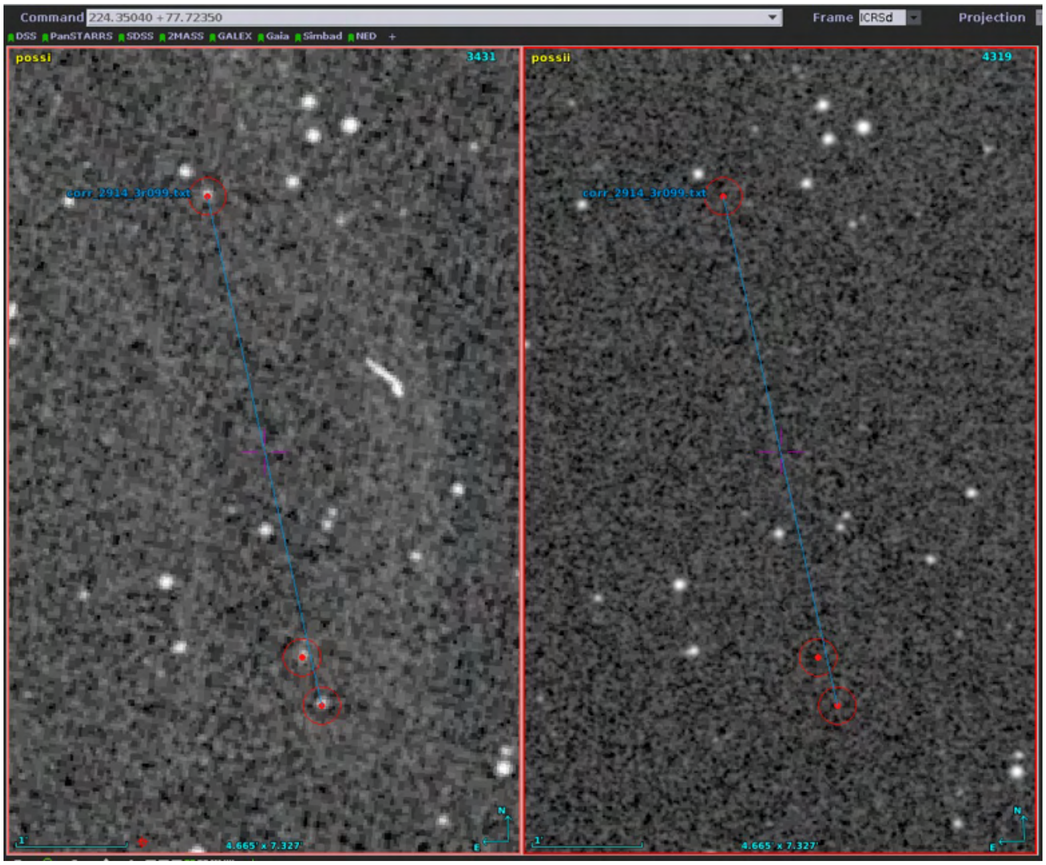


**Figure 32**

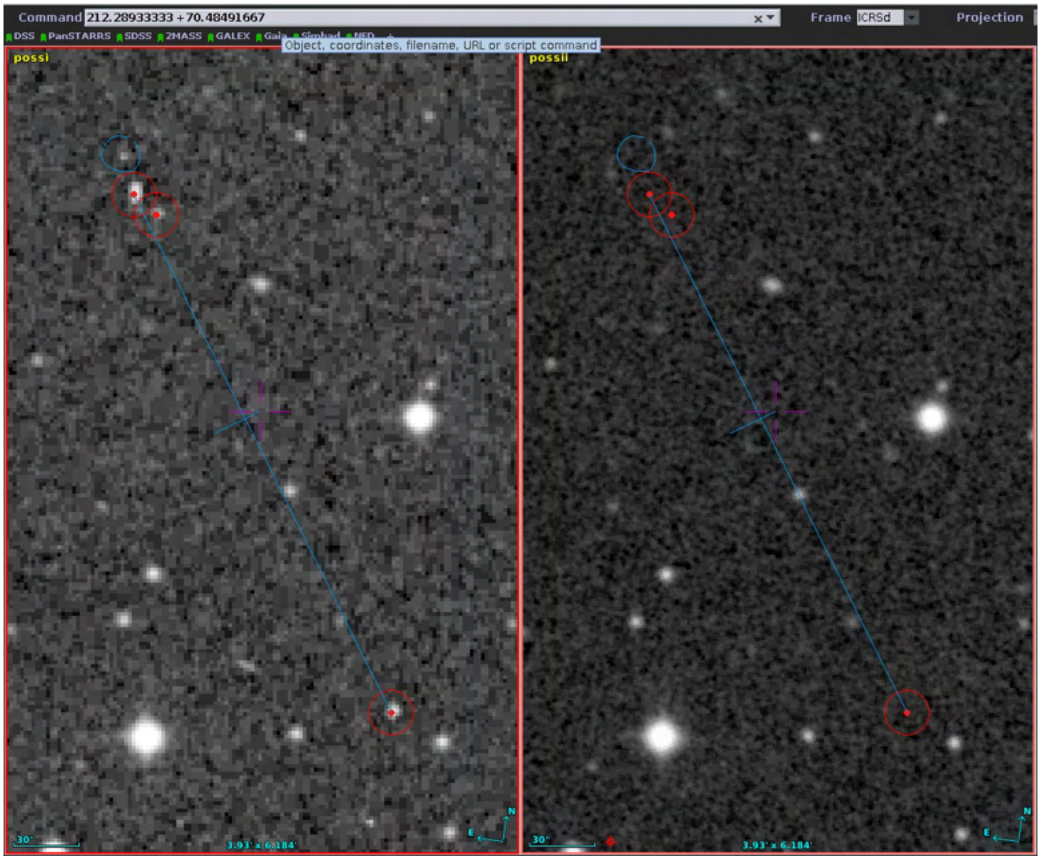


**Figure 33**

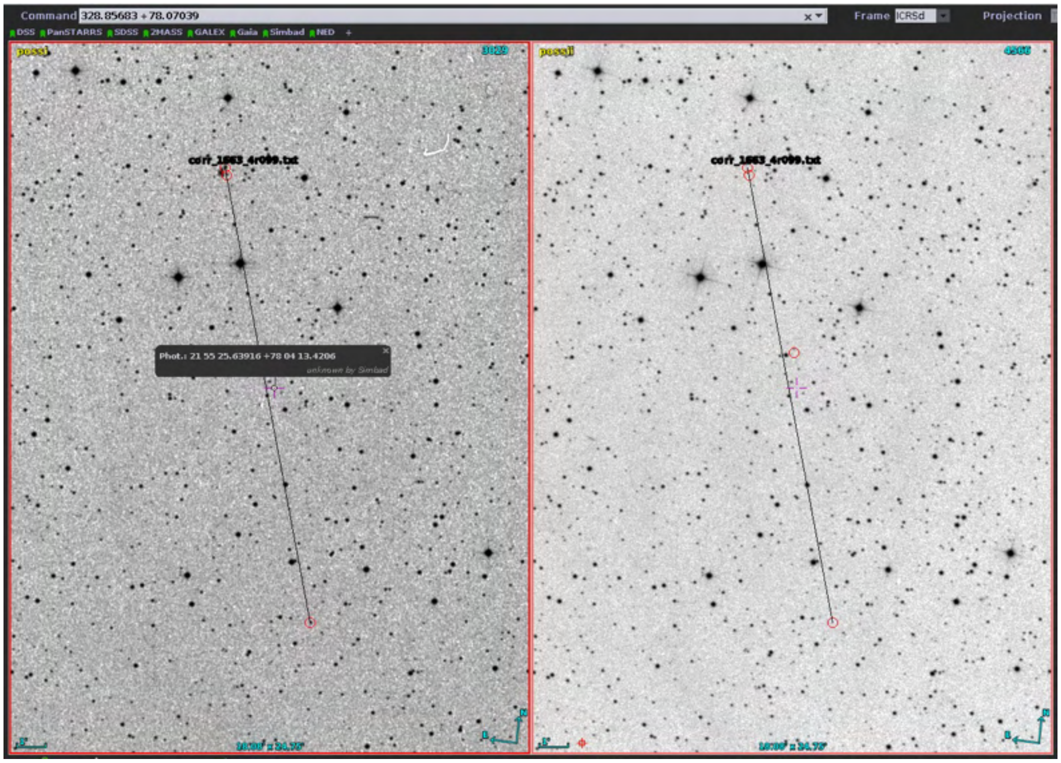


**Figure 34**

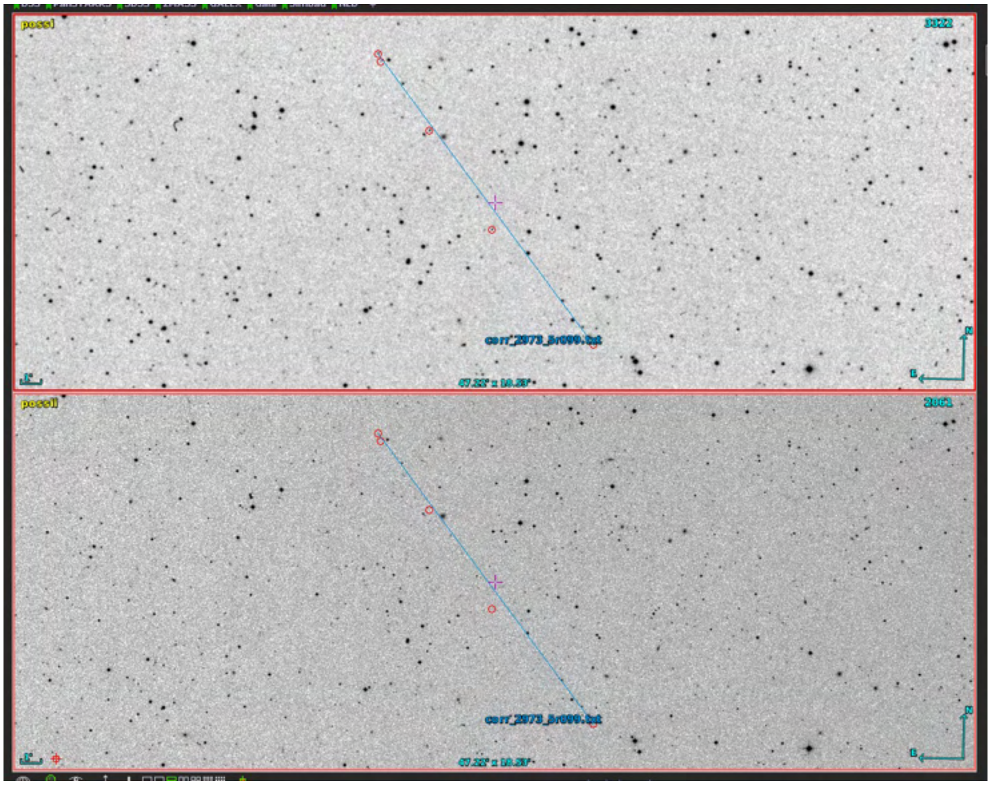

**Figure 35**

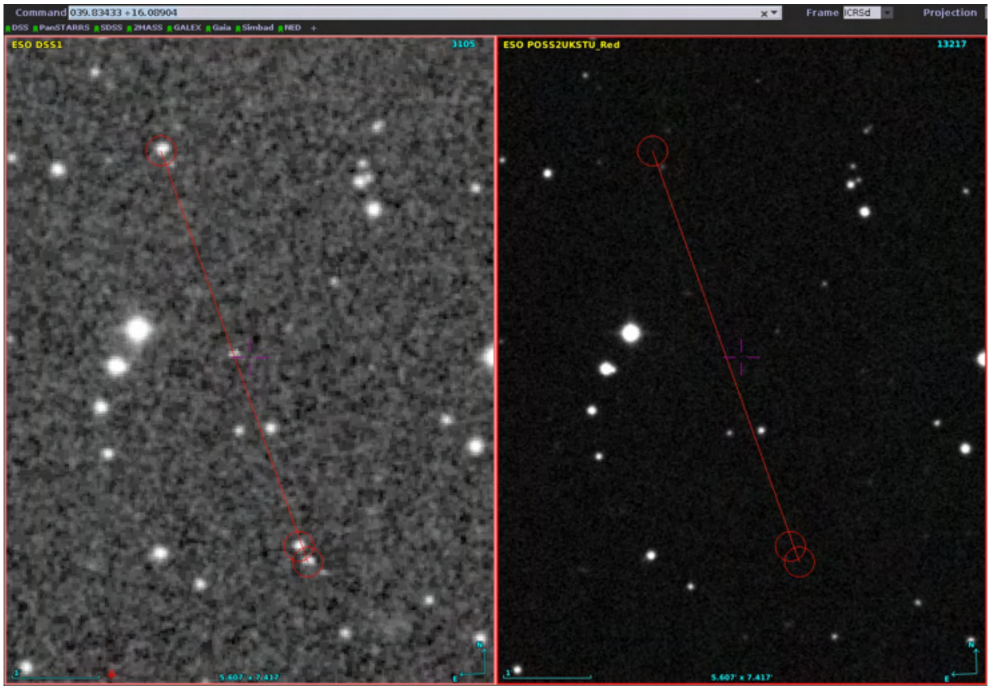


**Figure 36**

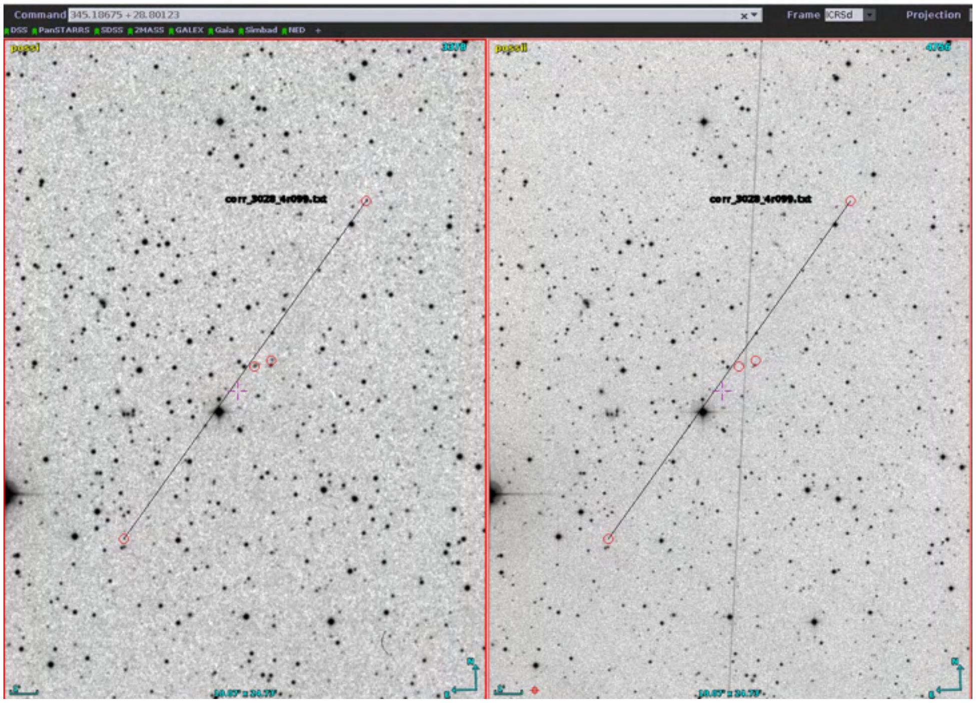


Figure 37

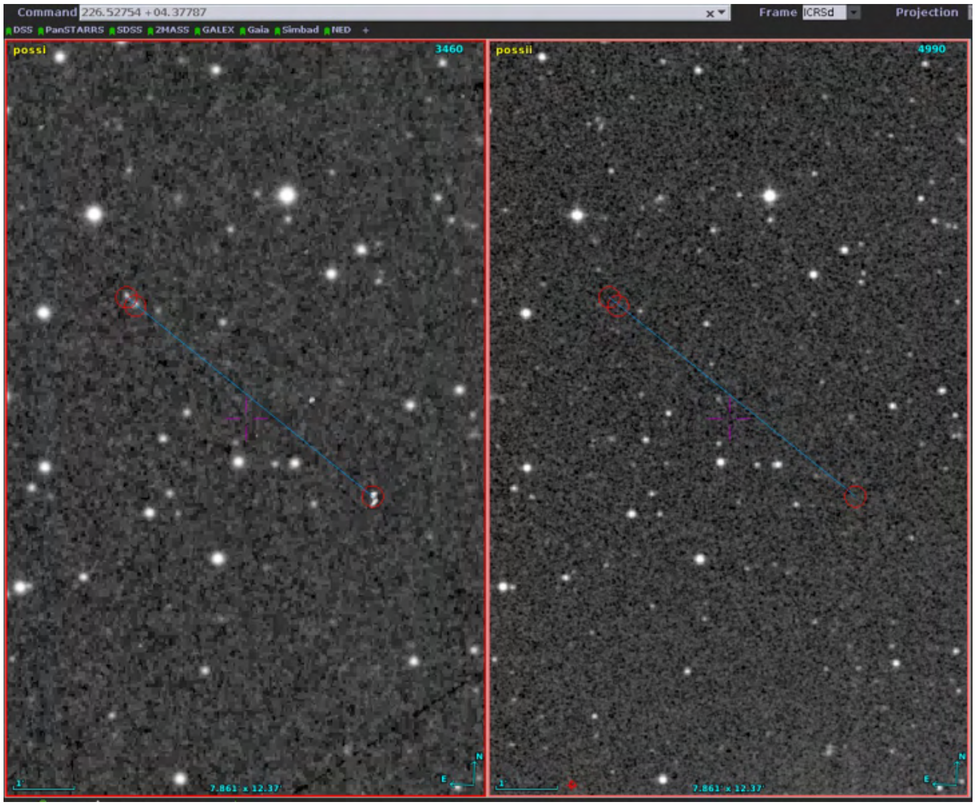


Figure 38

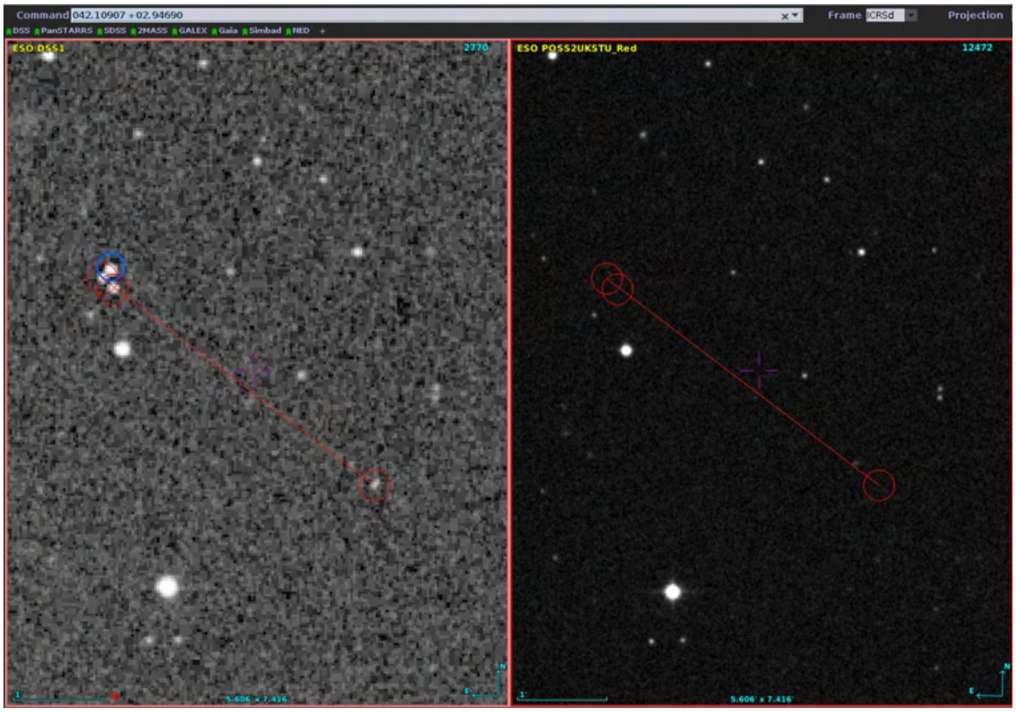


Figure 39

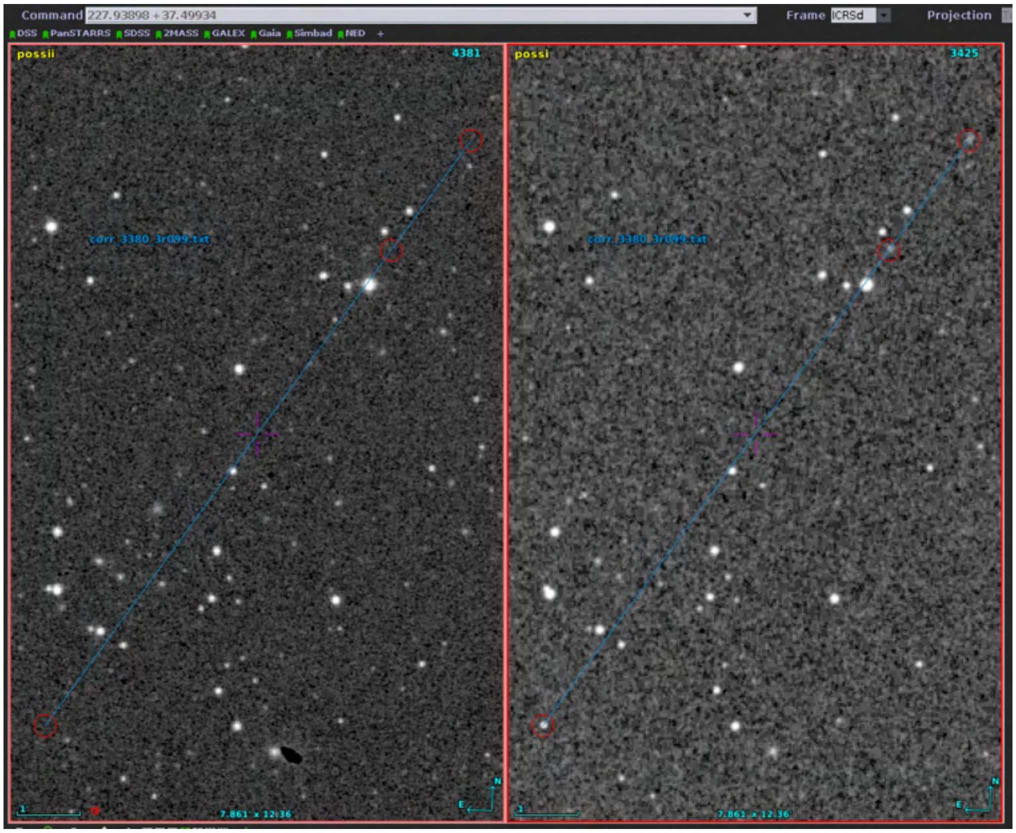


Figure 40

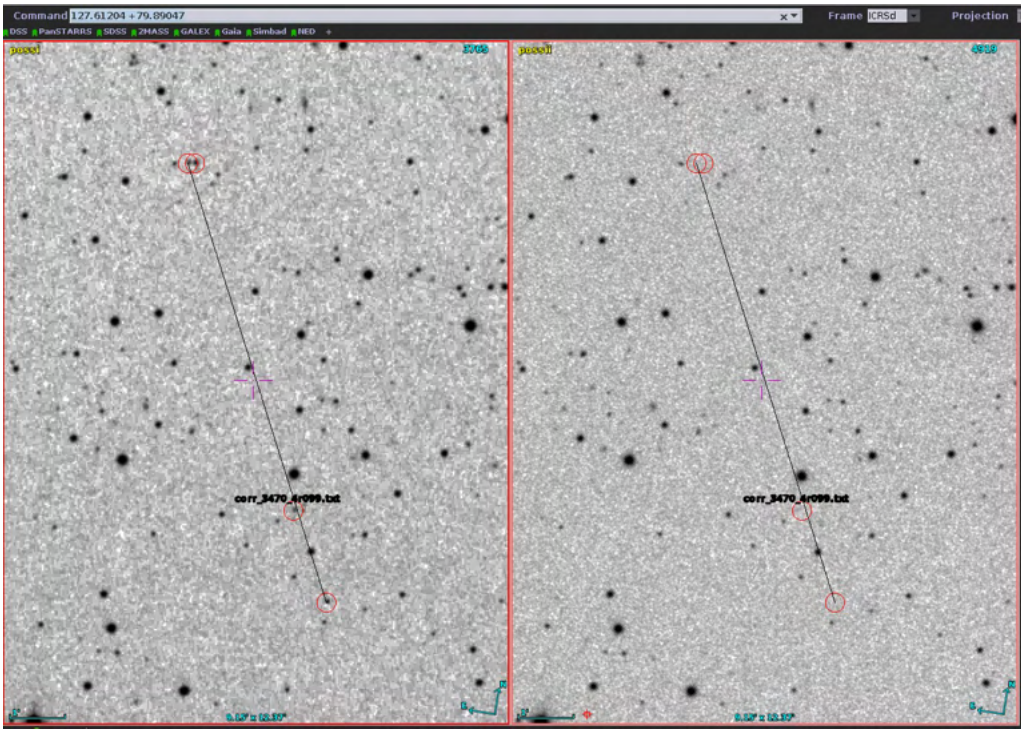


**Figure 41**

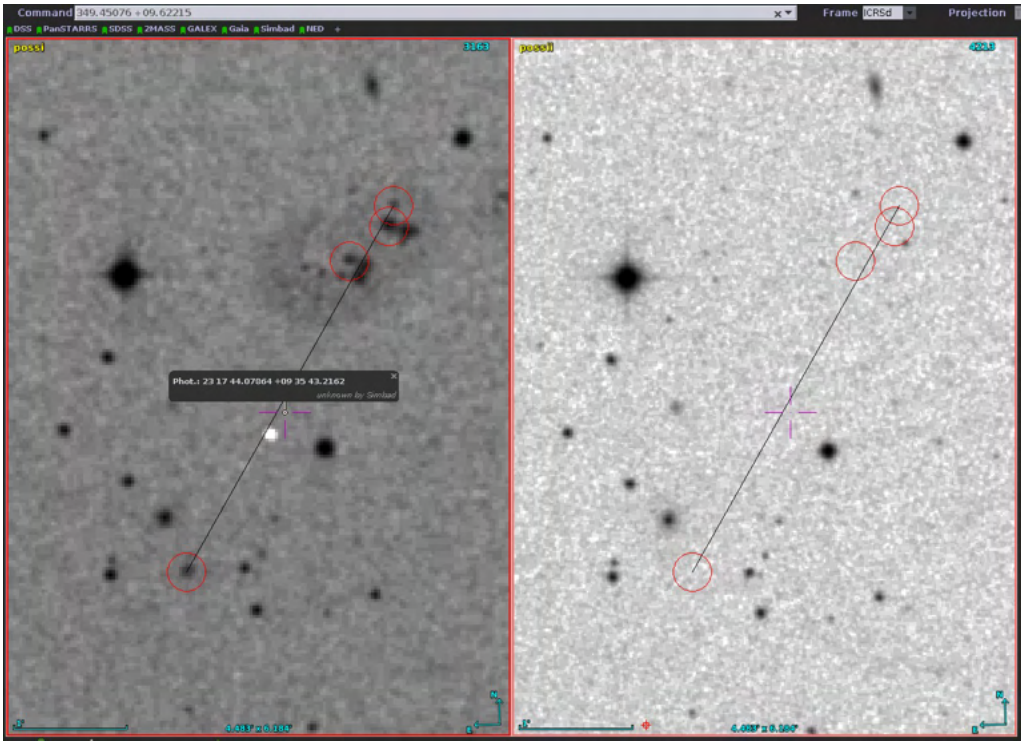


**Figure 42**

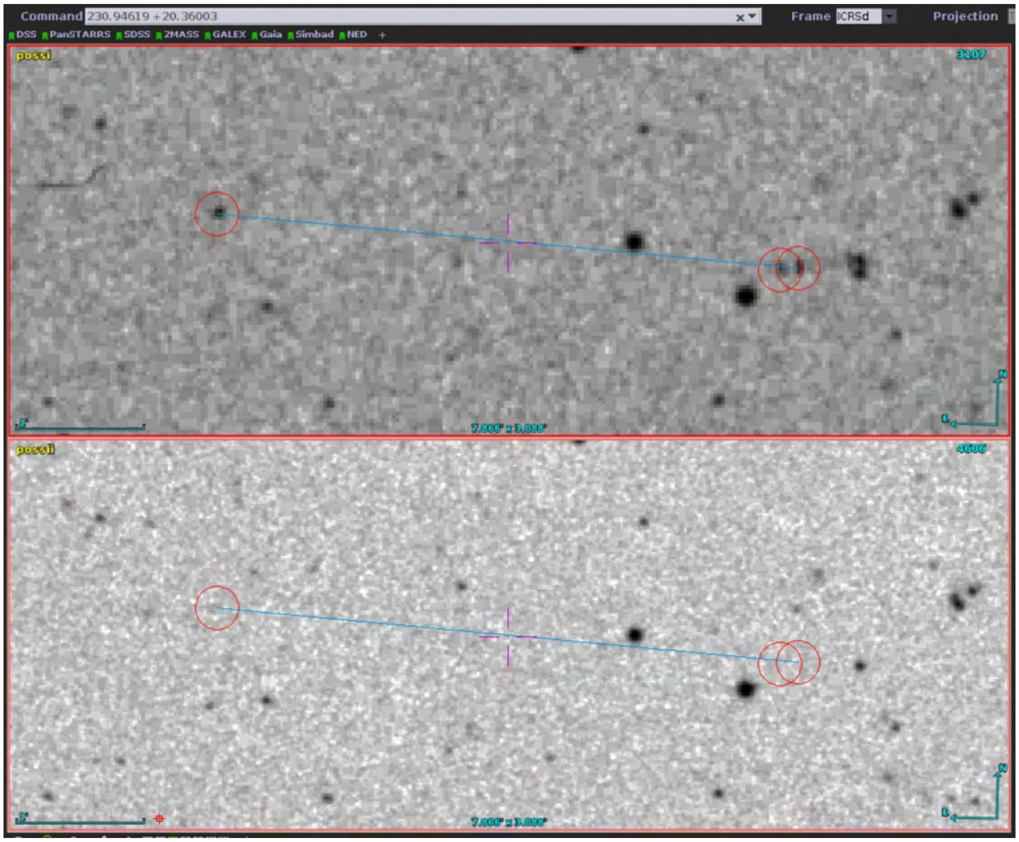


Figure 43

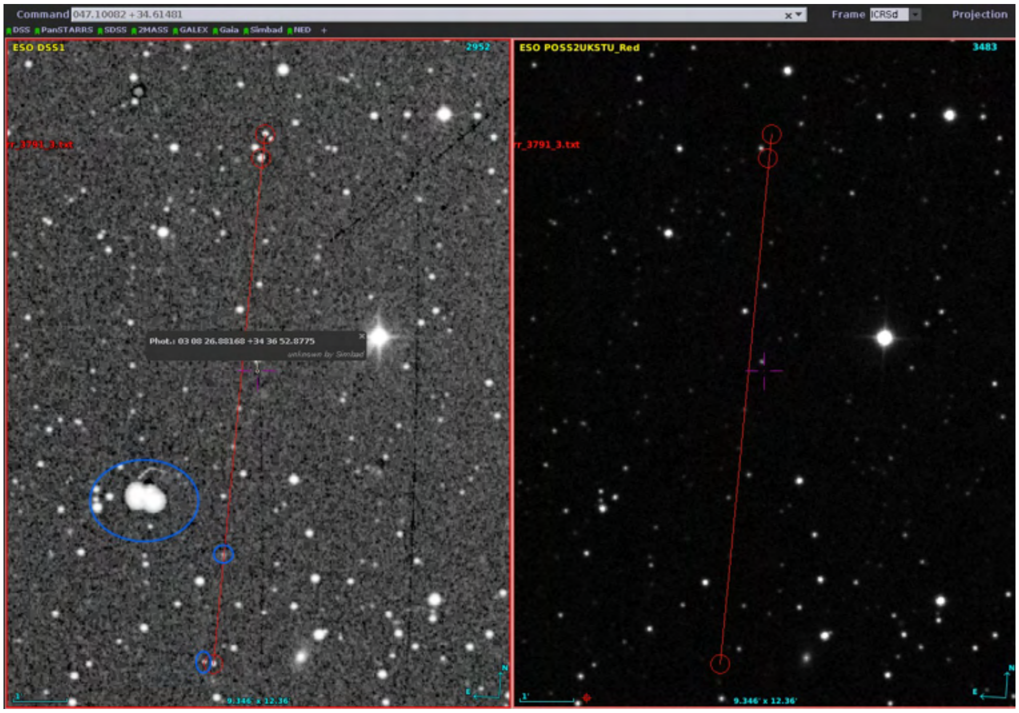


Figure 44

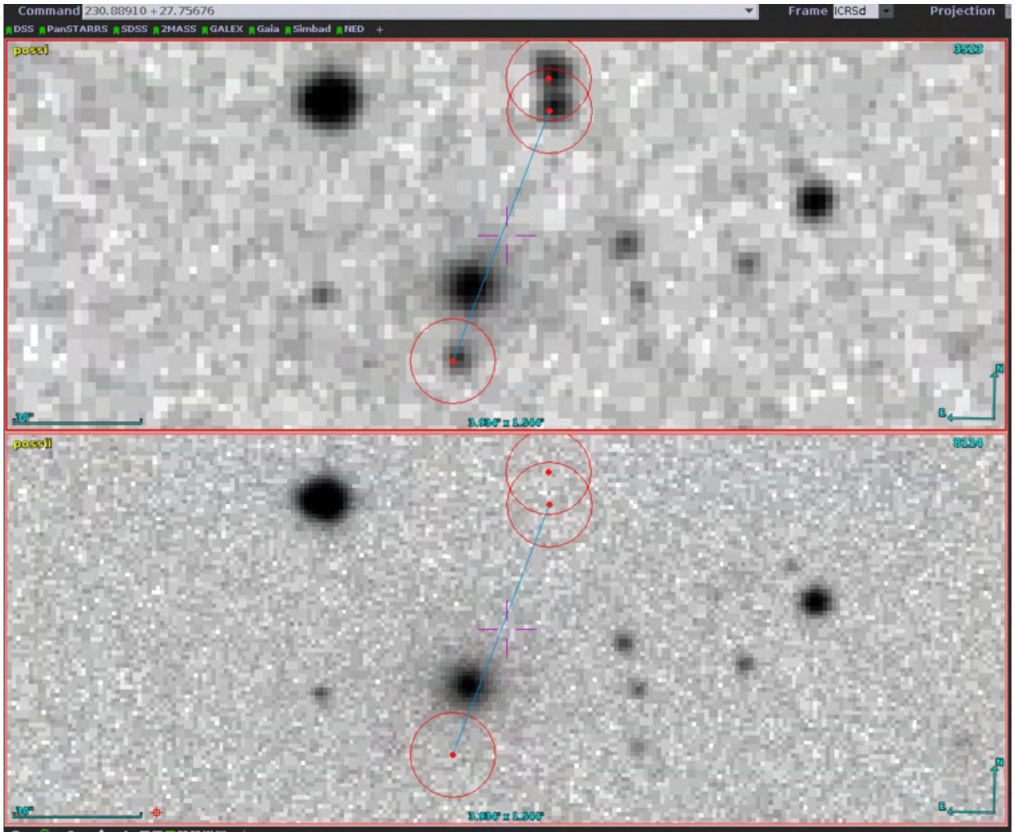


**Figure 45**

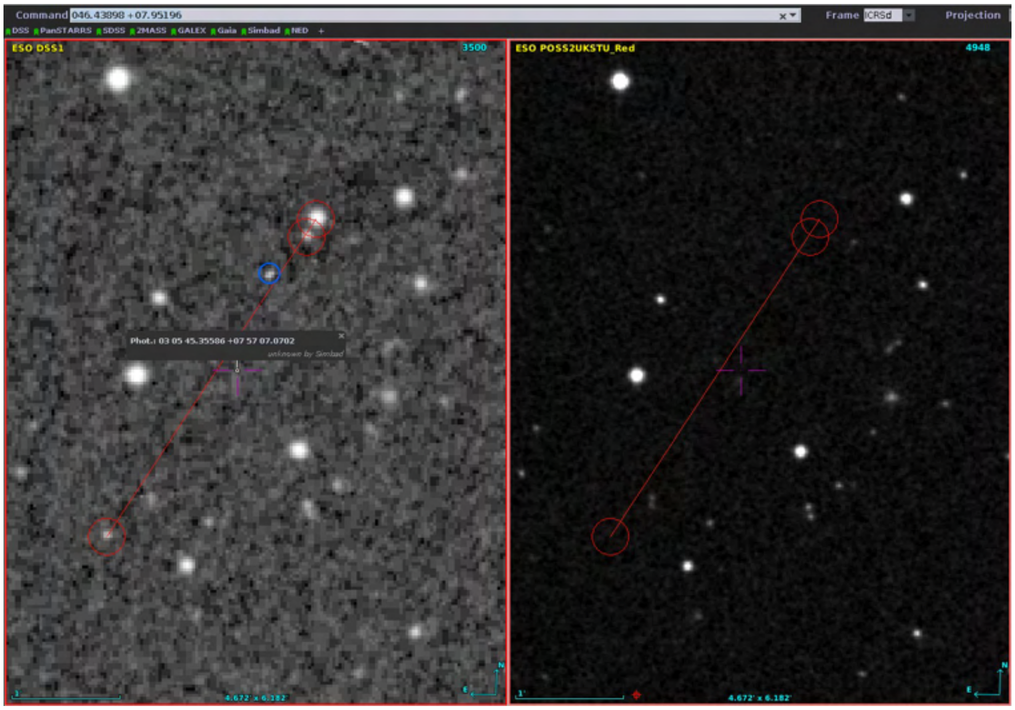


**Figure 46**

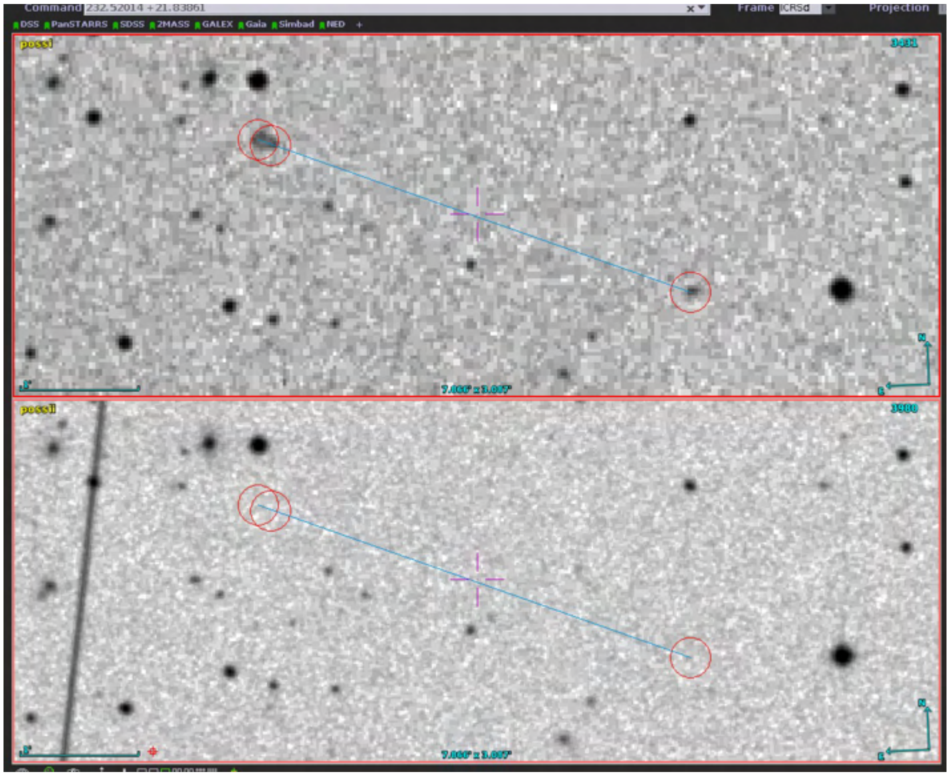


Figure 47

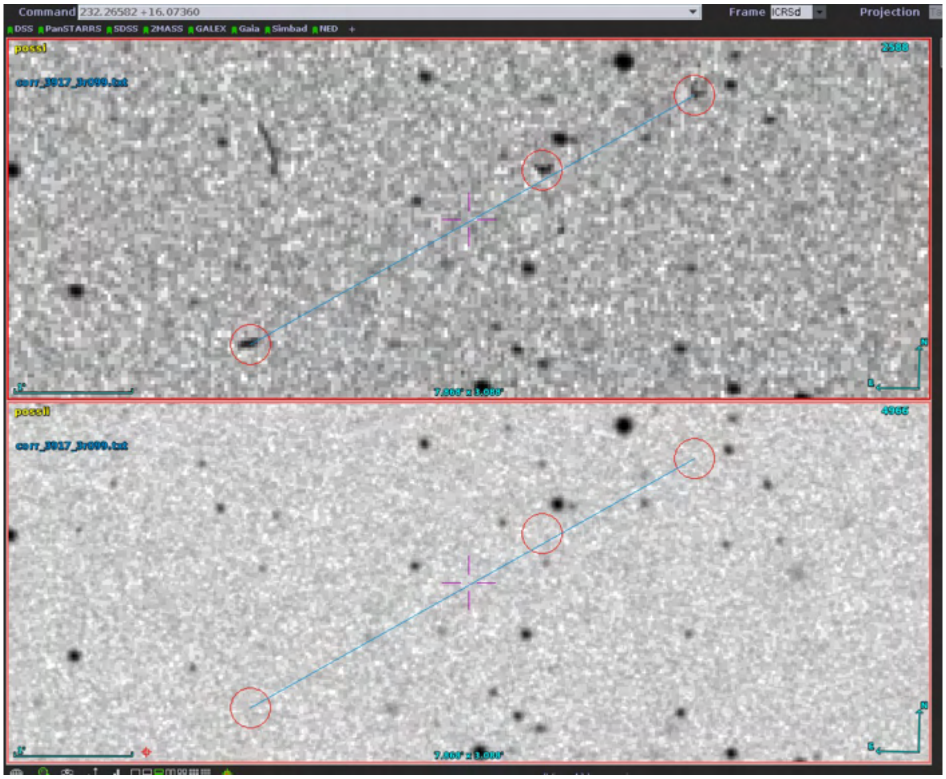


Figure 48

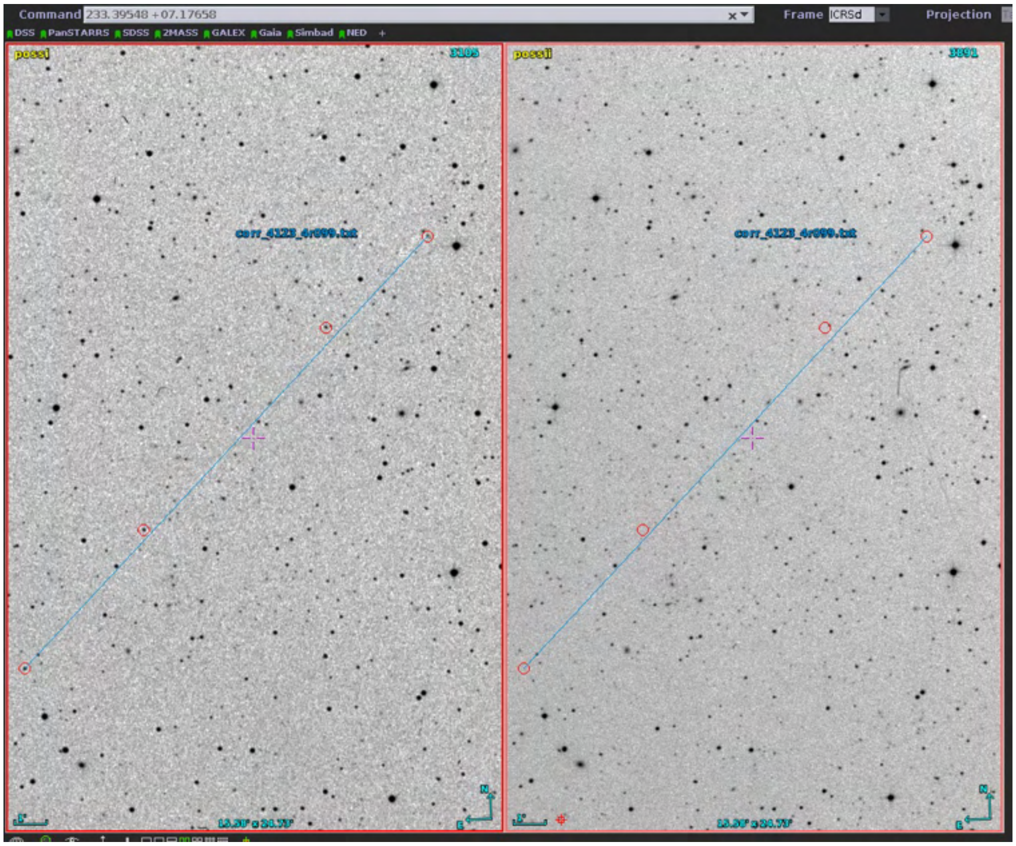


**Figure 49**

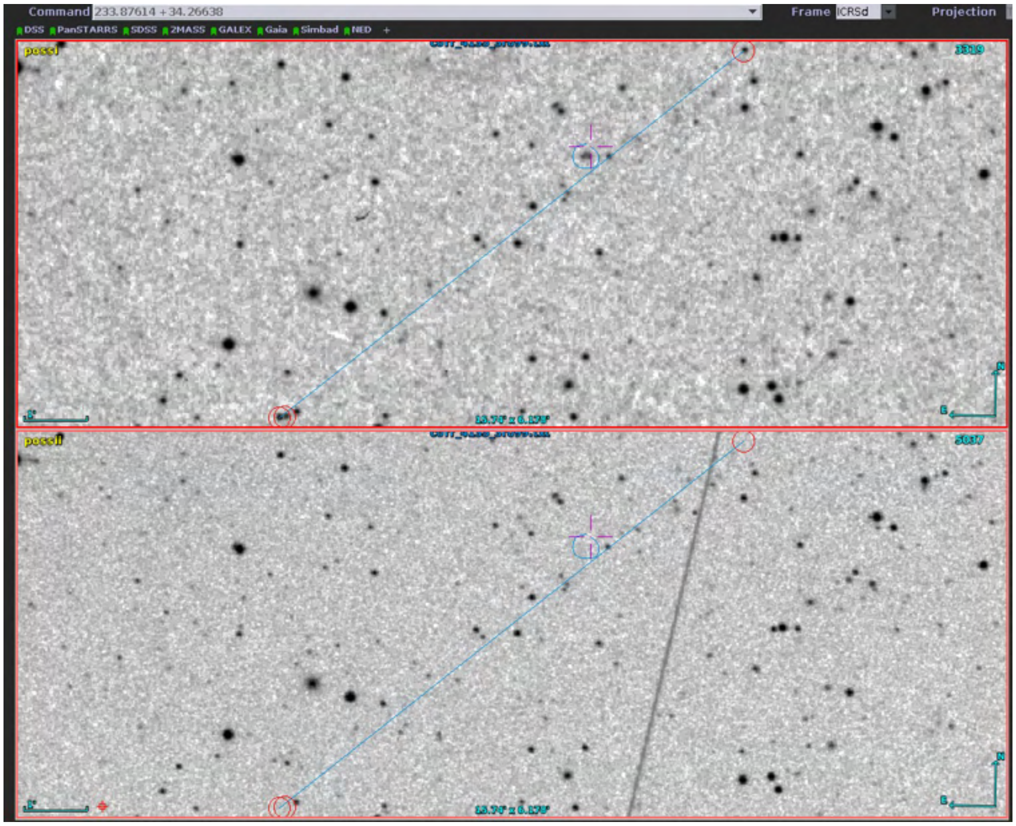


**Figure 50**

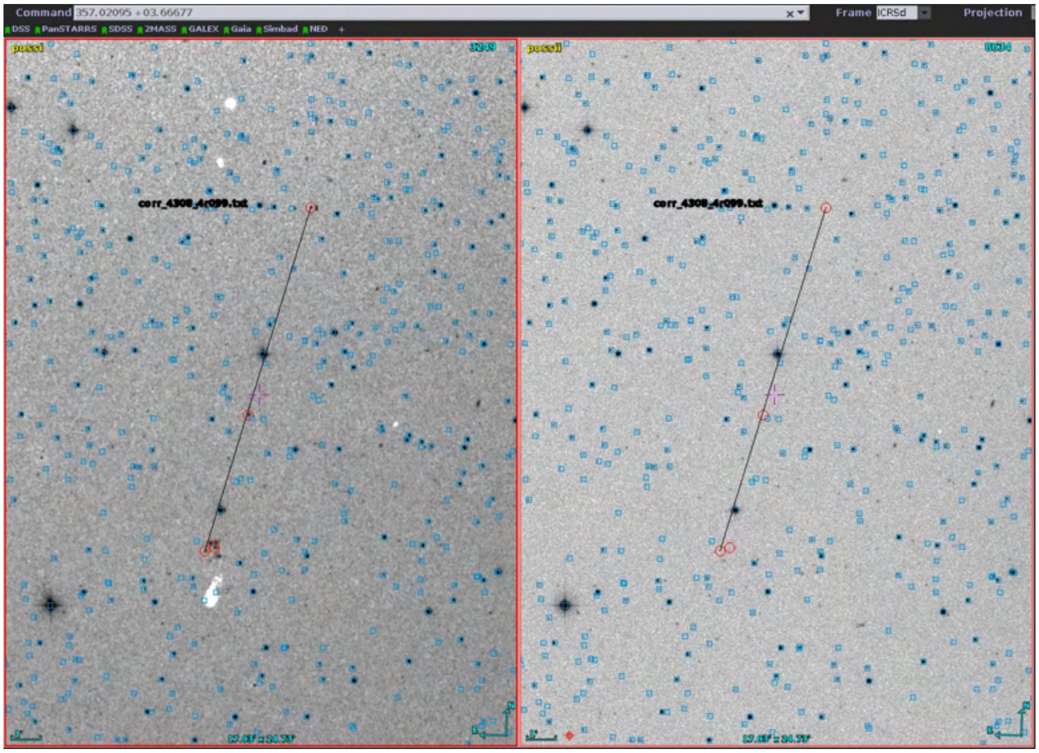


**Figure 51**

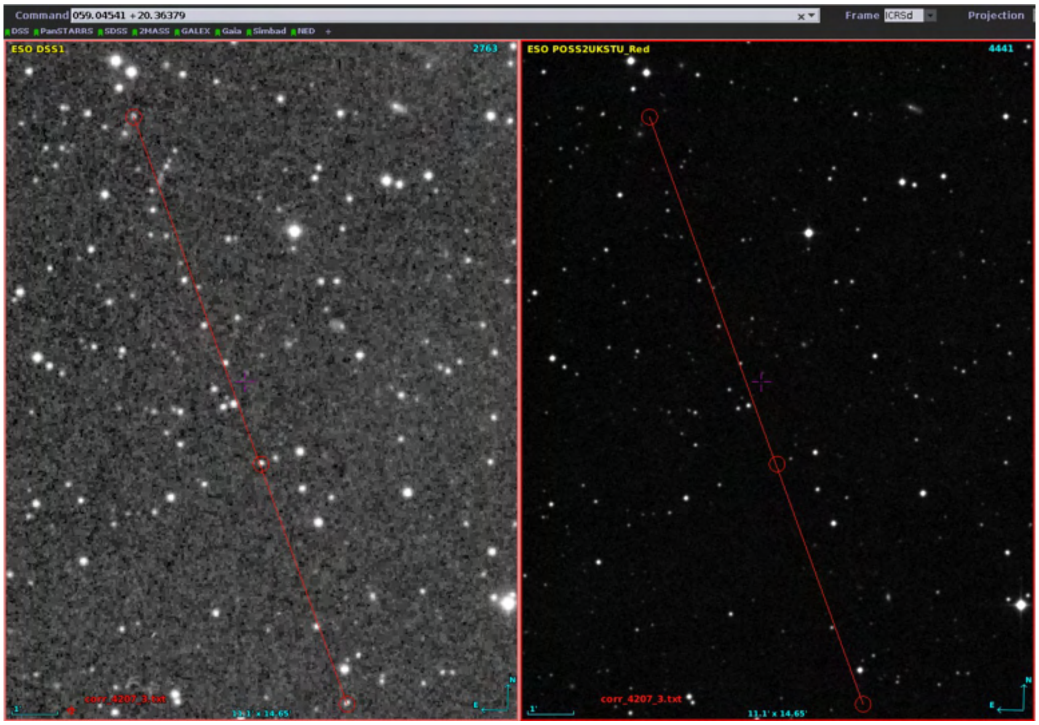


**Figure 52**

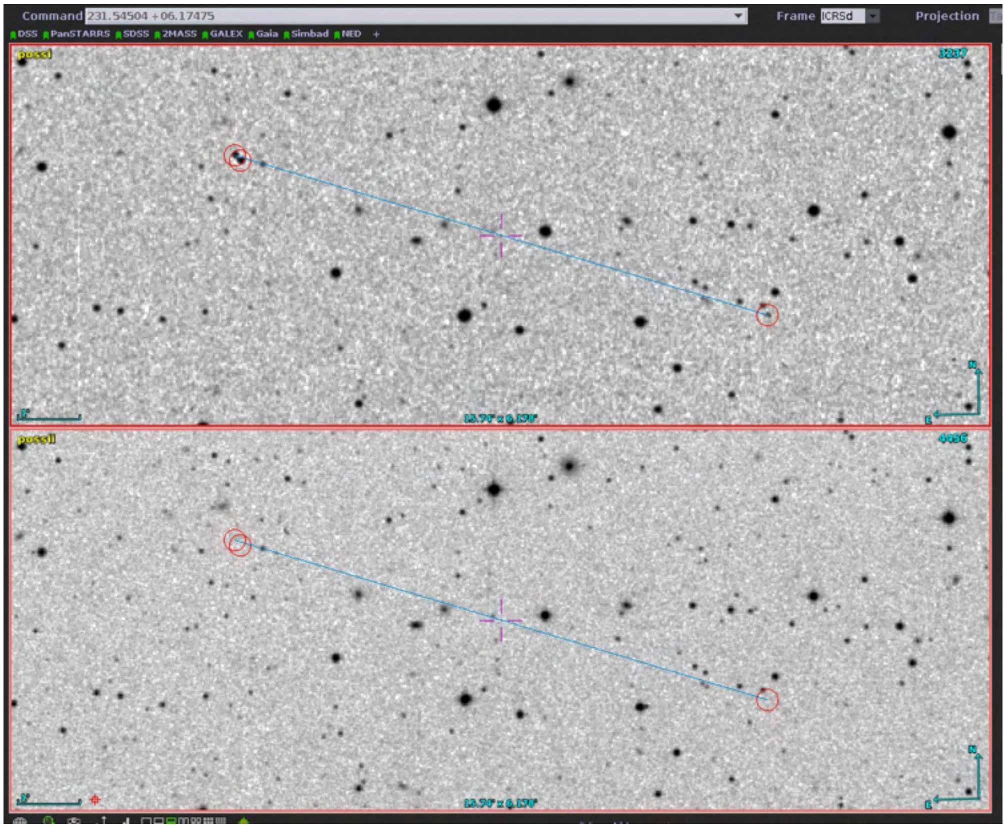


**Figure 53**

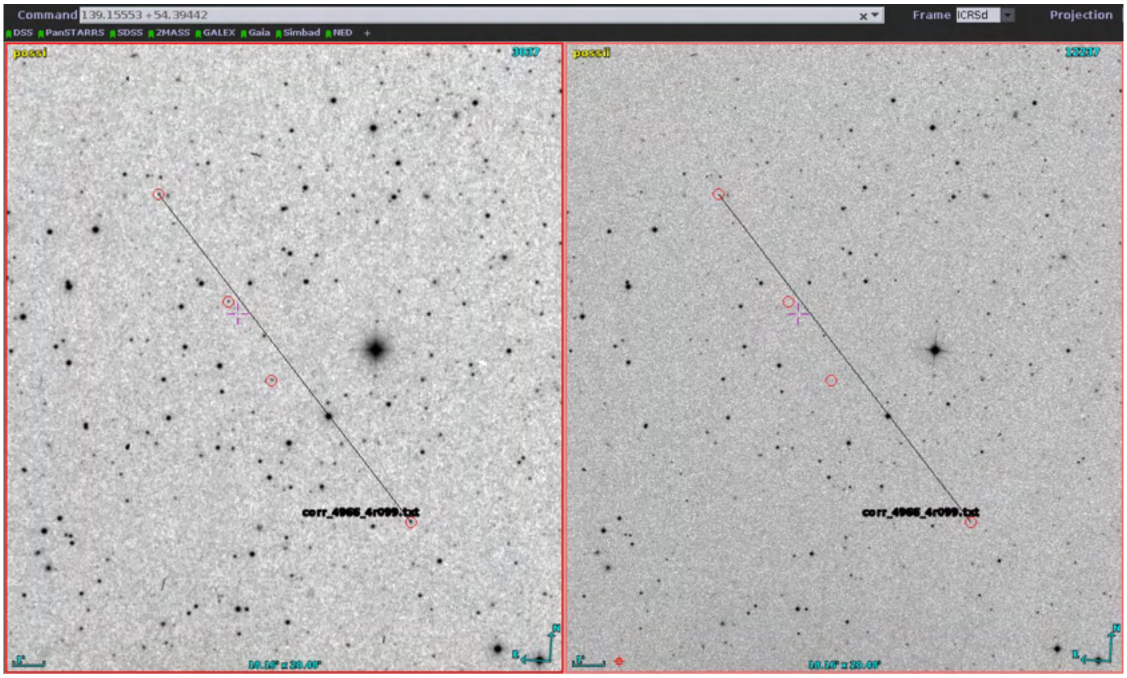


**Figure 54**

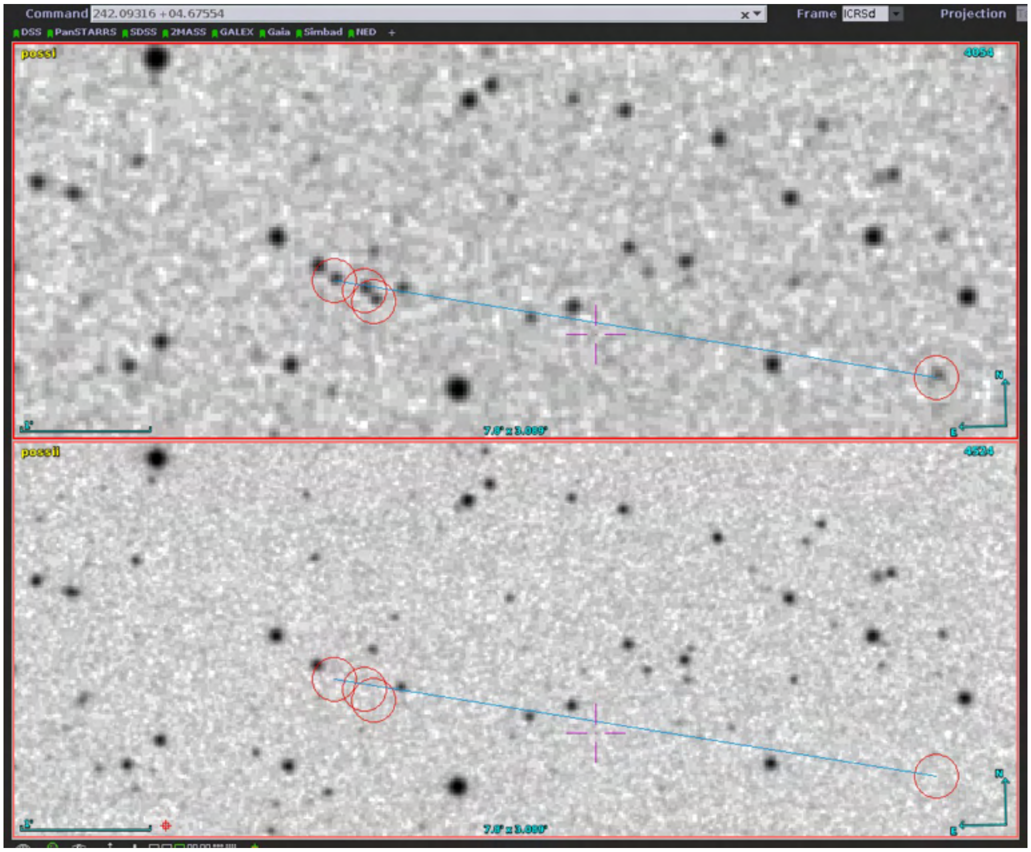


Figure 55

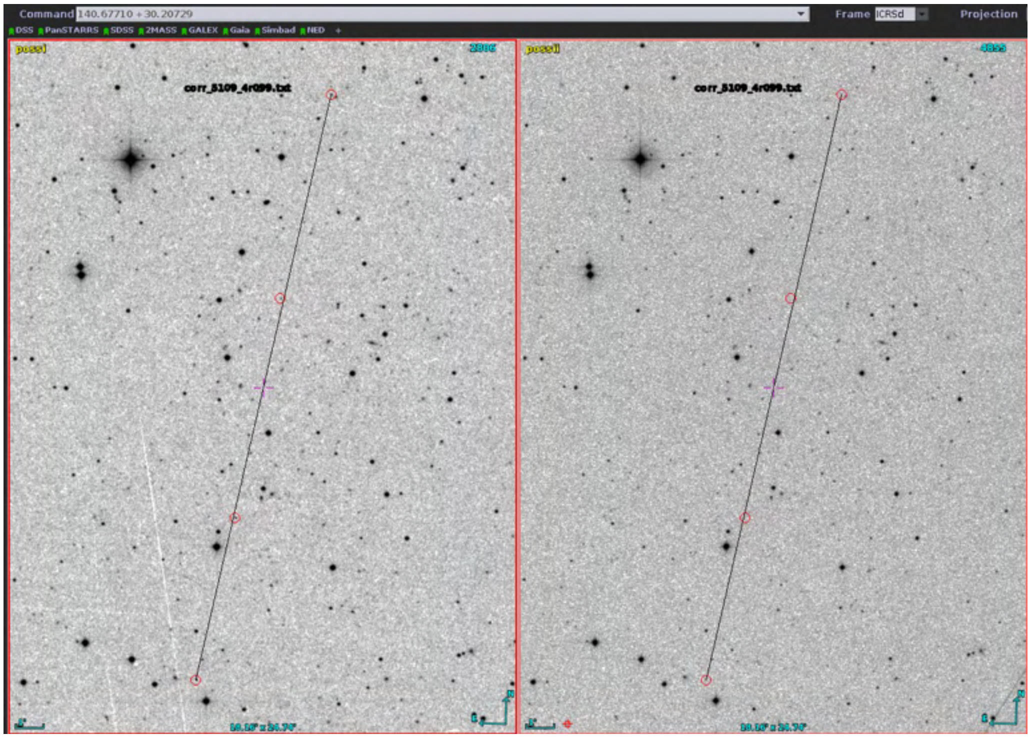


Figure 56

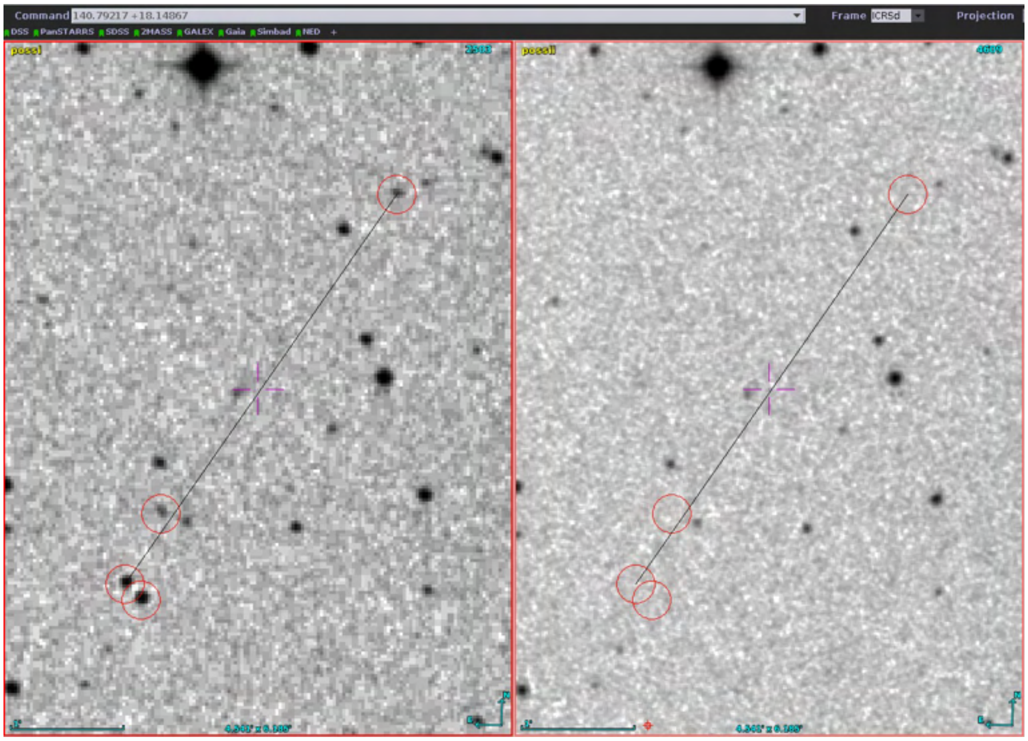


# Figure 57

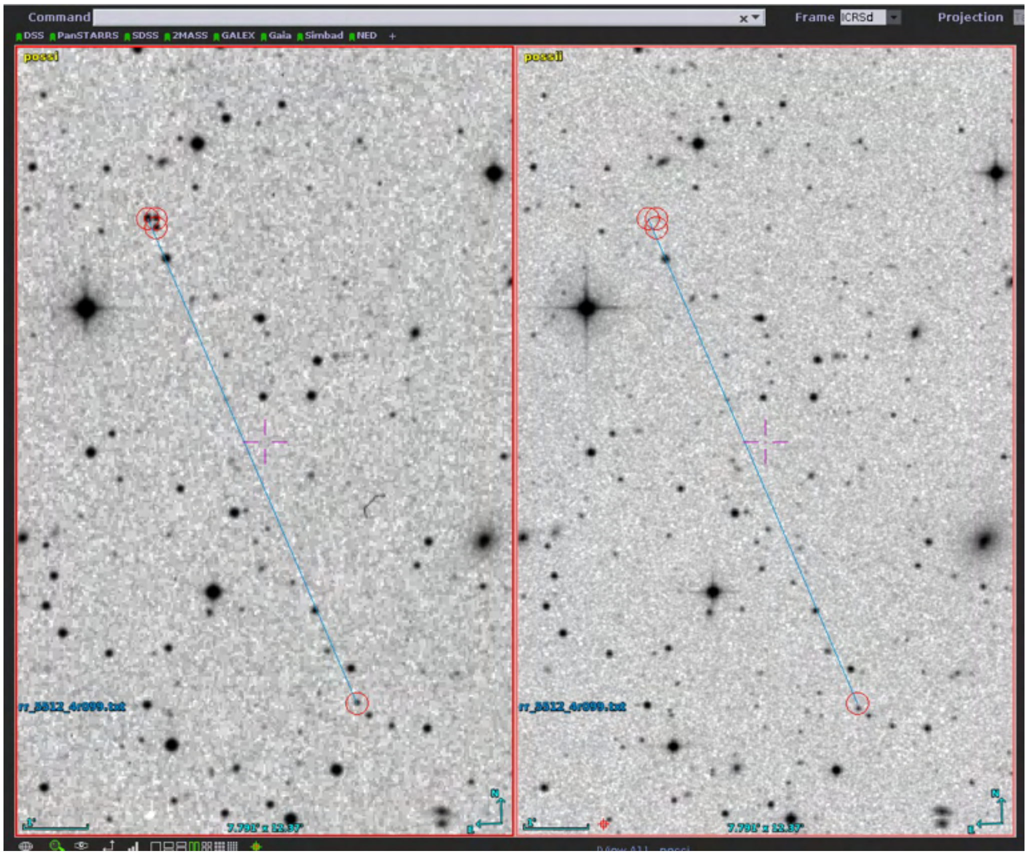


# Figure 58

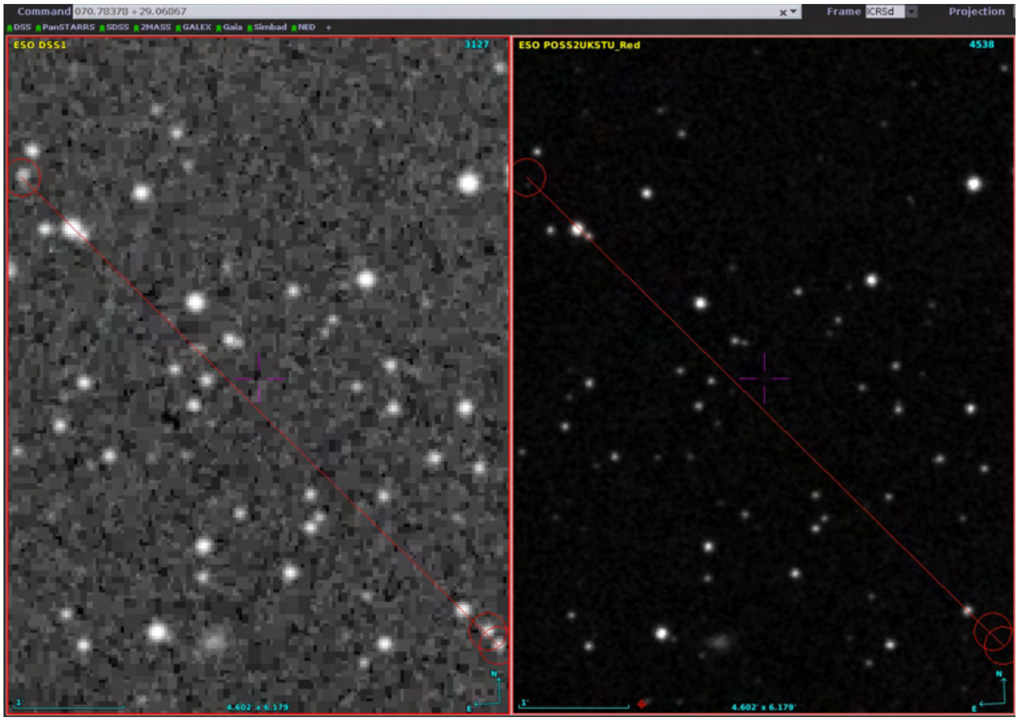


# Figure 59

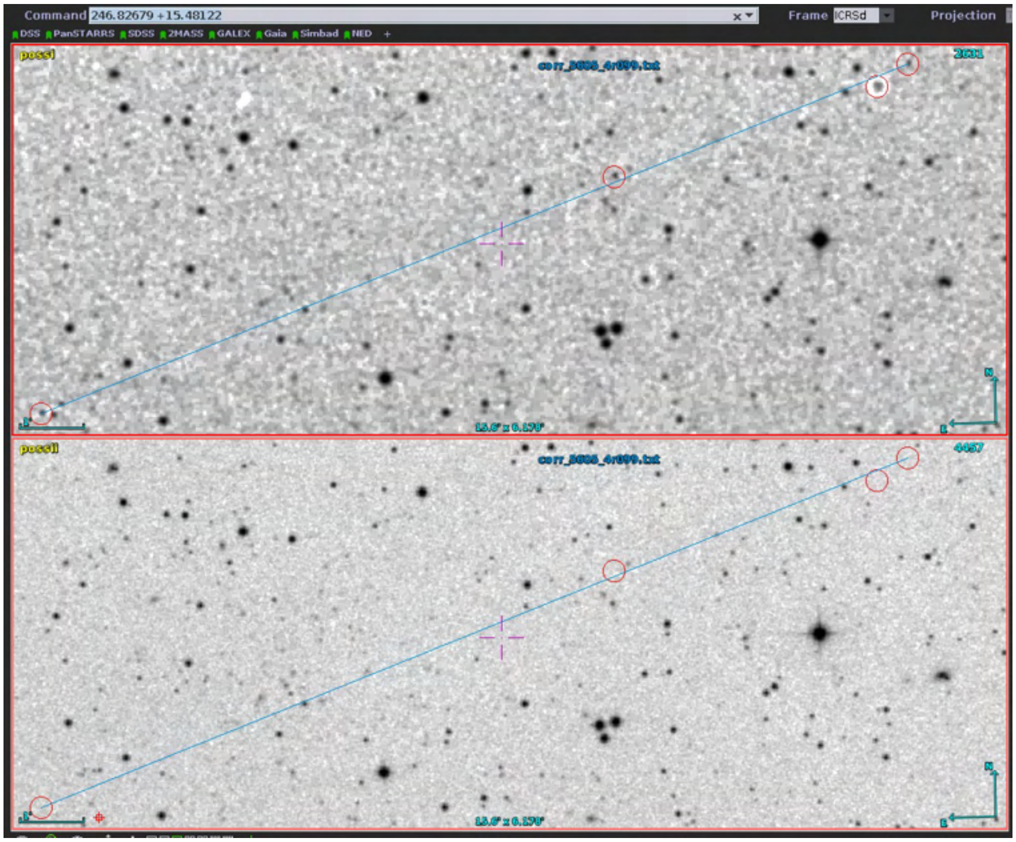


# Figure 60

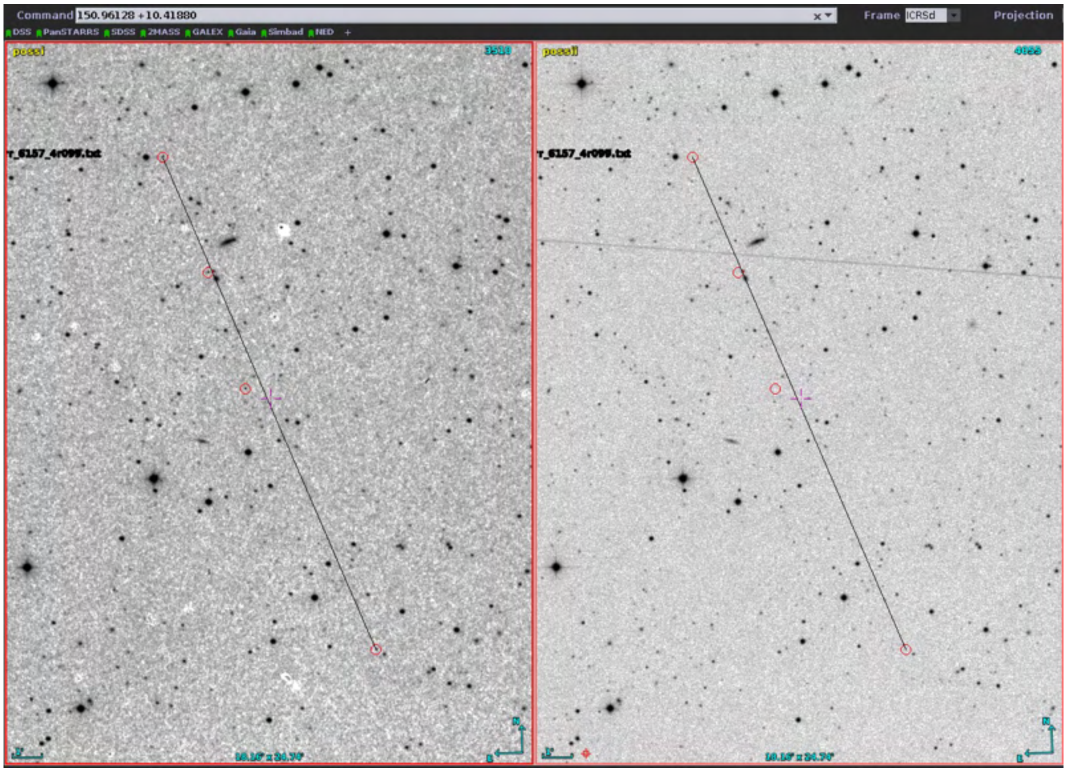


Figure 61

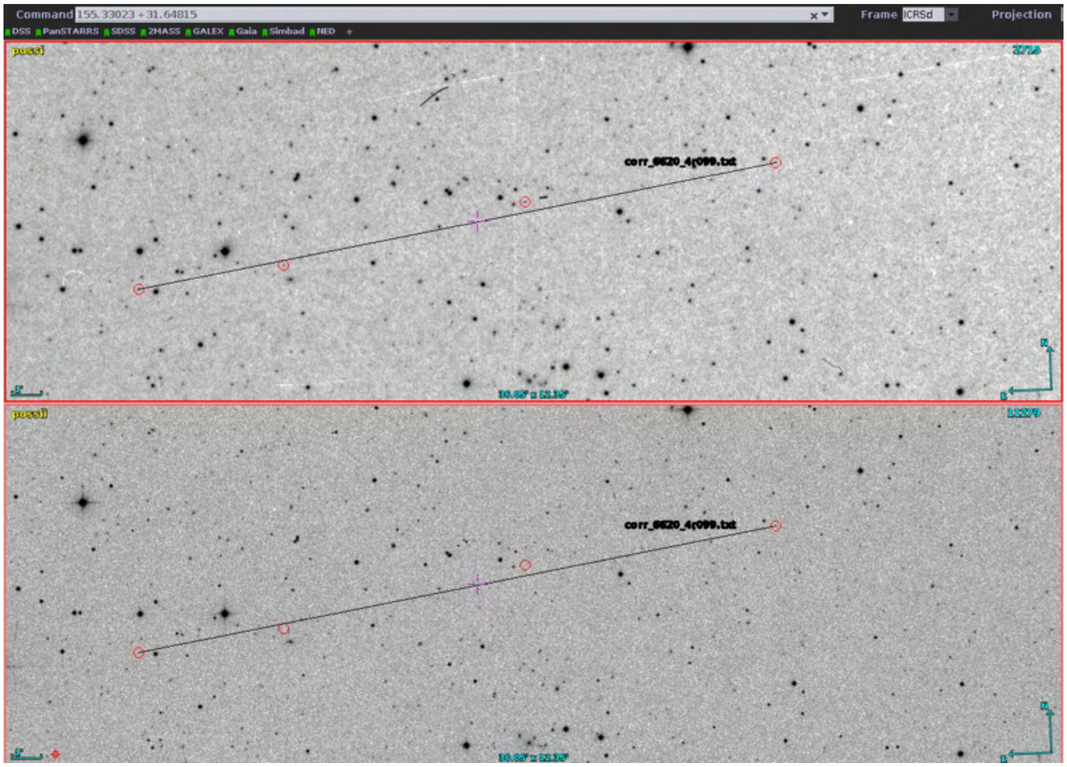


Figure 62

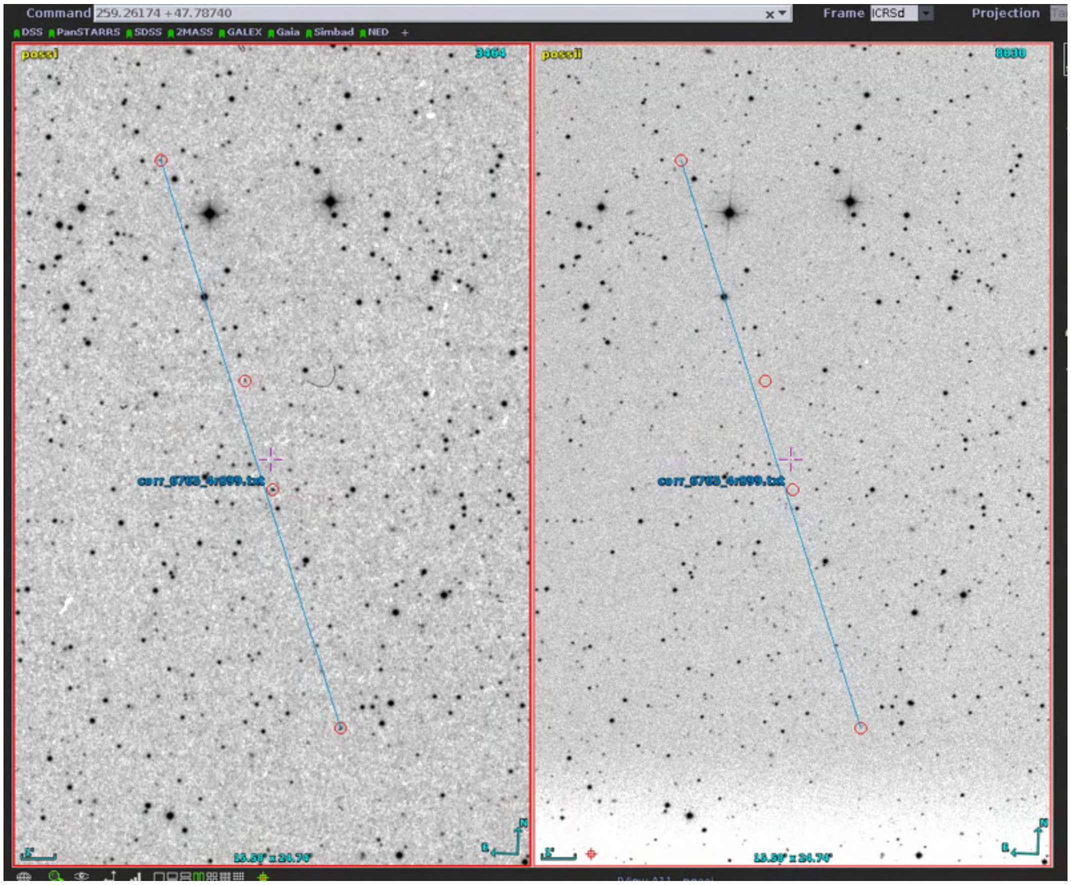


**Figure 63**

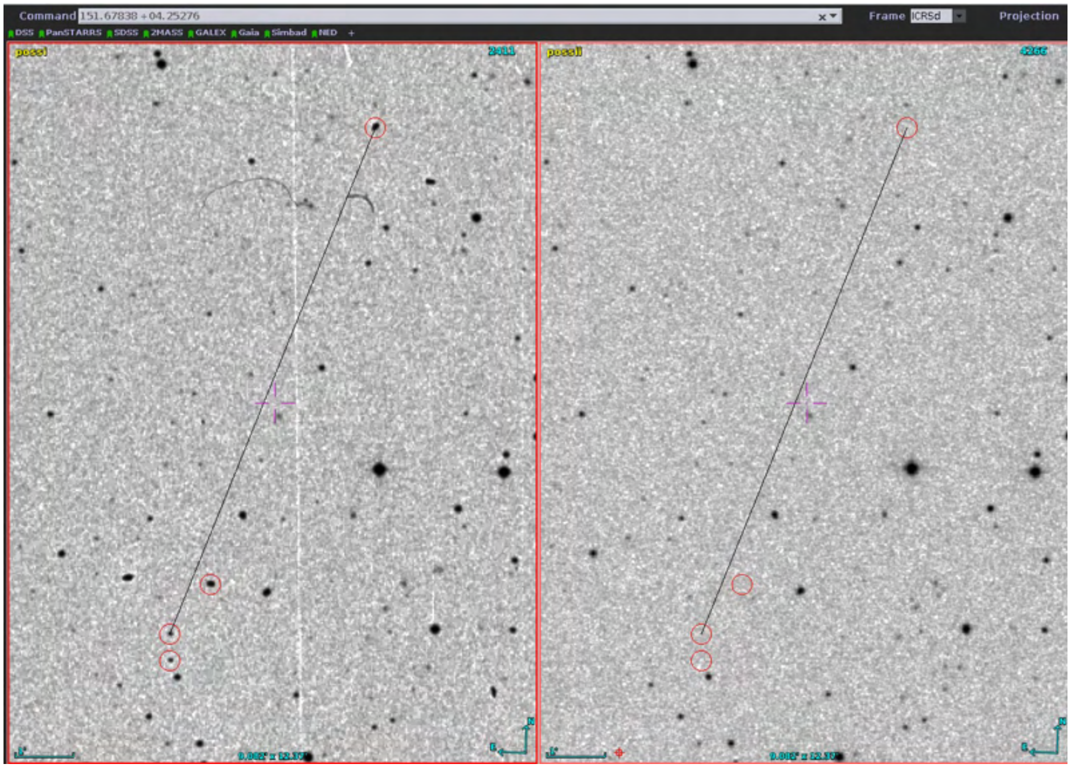


**Figure 64**

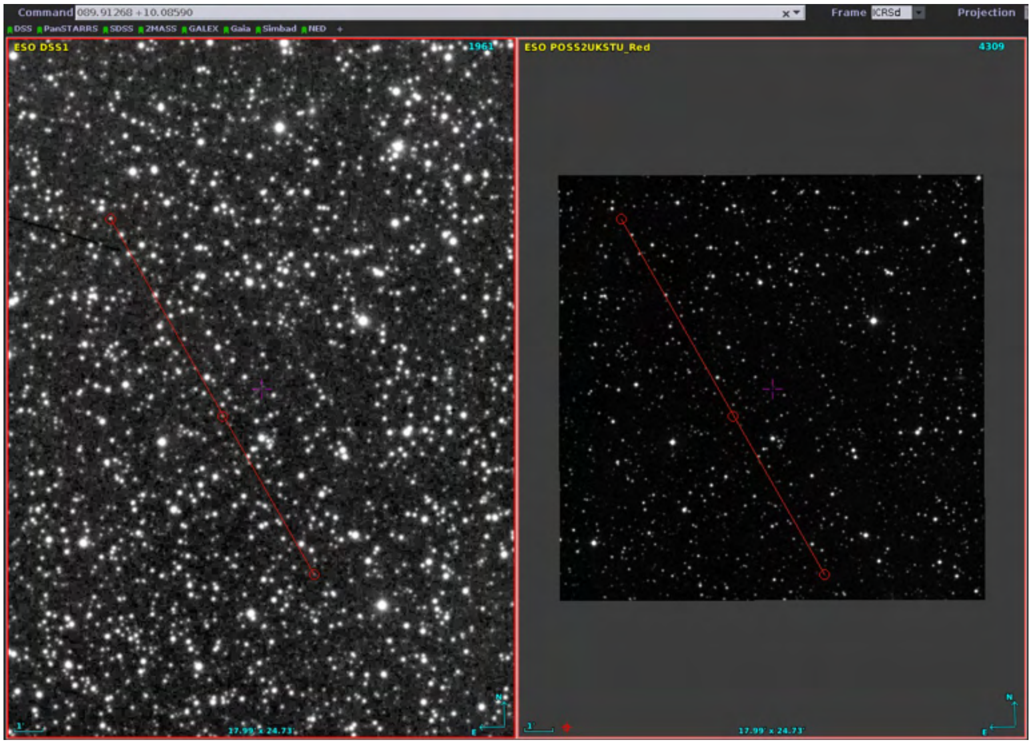


**Figure 65**

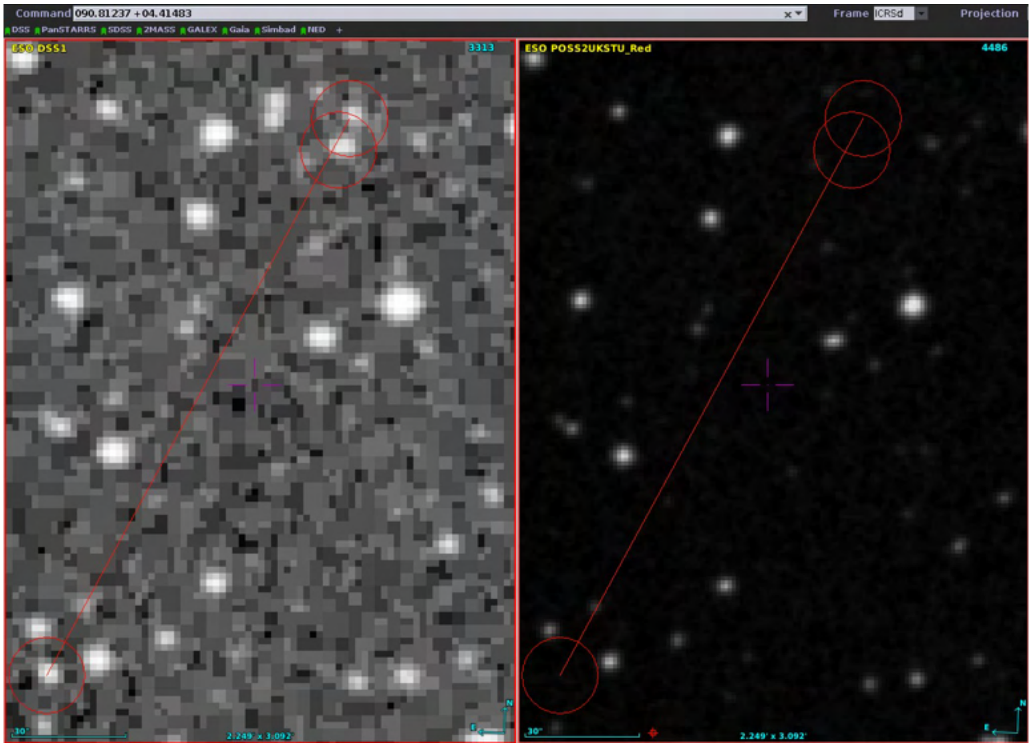


**Figure 66**

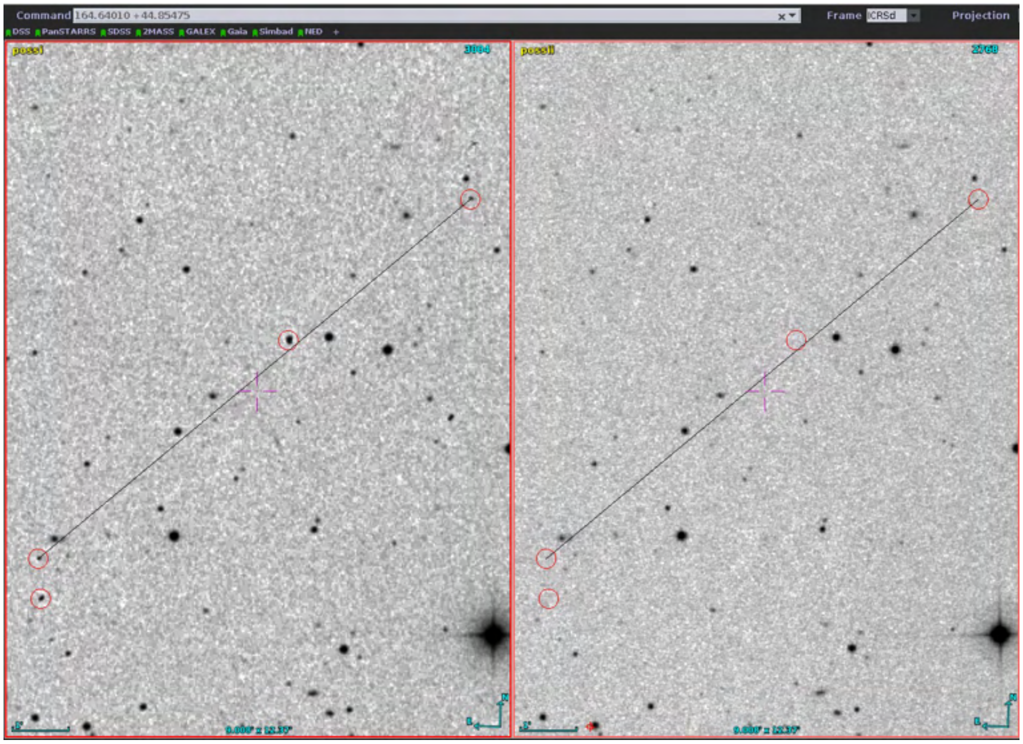


**Figure 67**

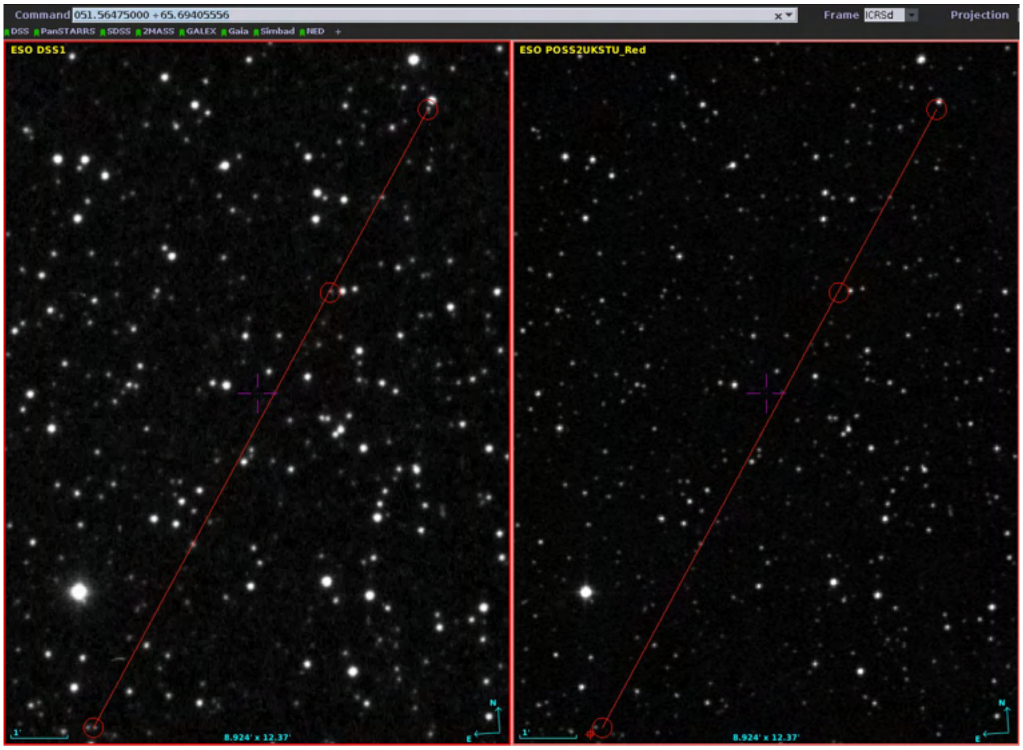


**Figure 68**

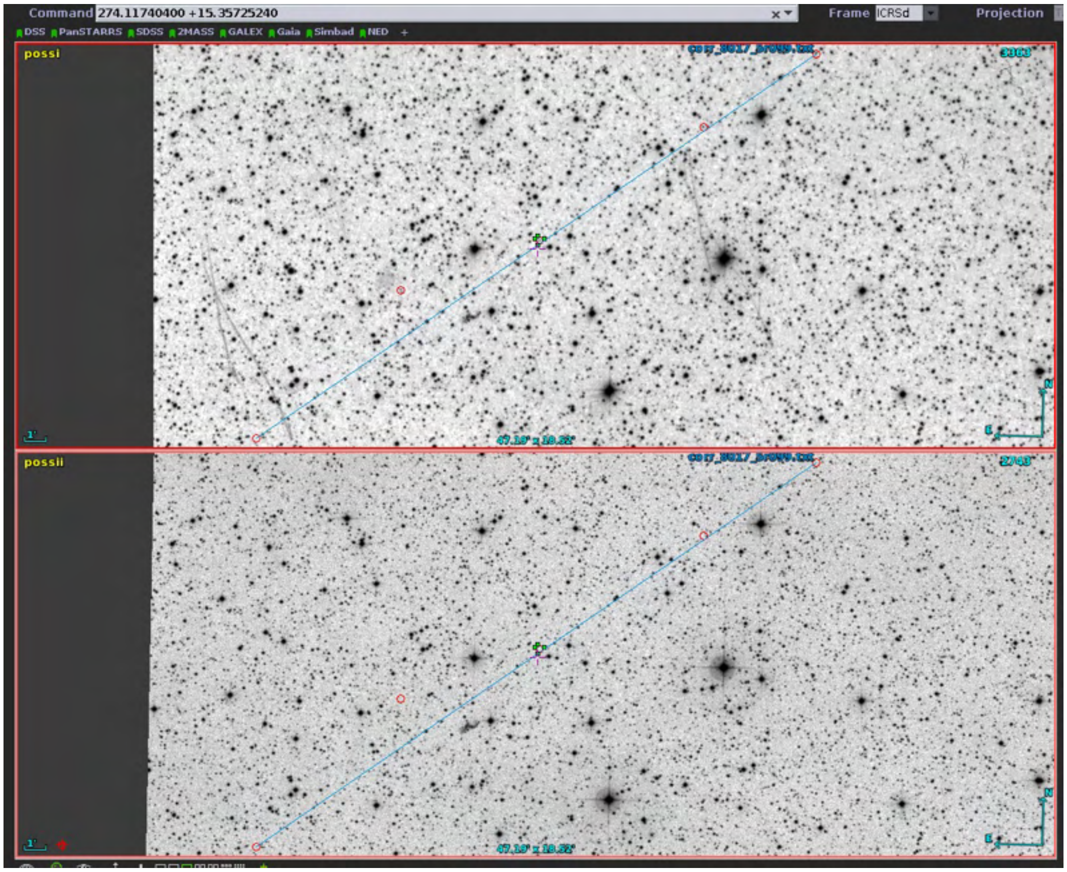


Figure 69

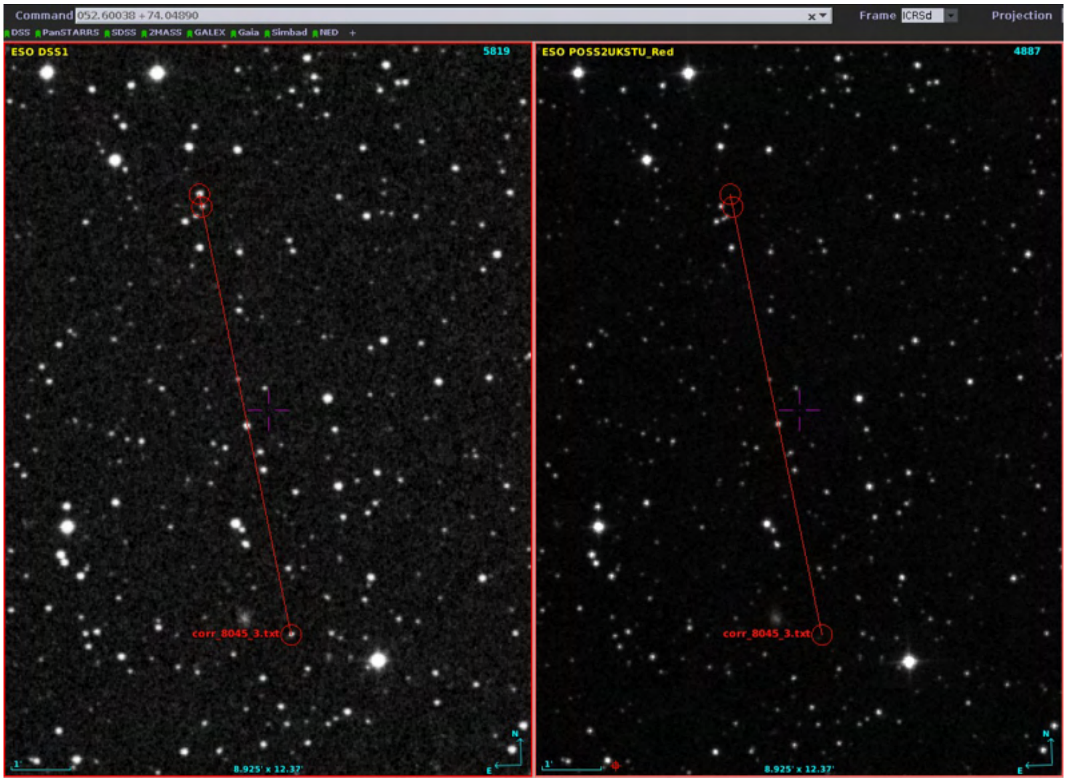


Figure 70

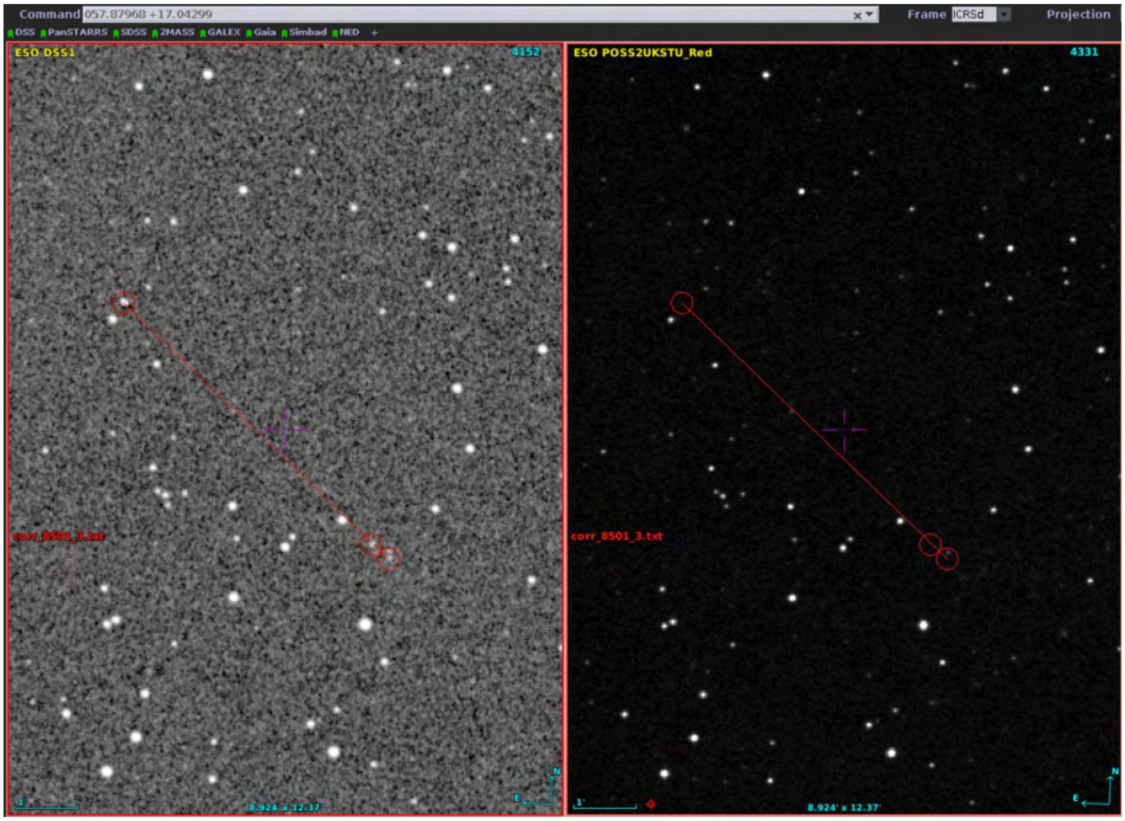


## Figure 71

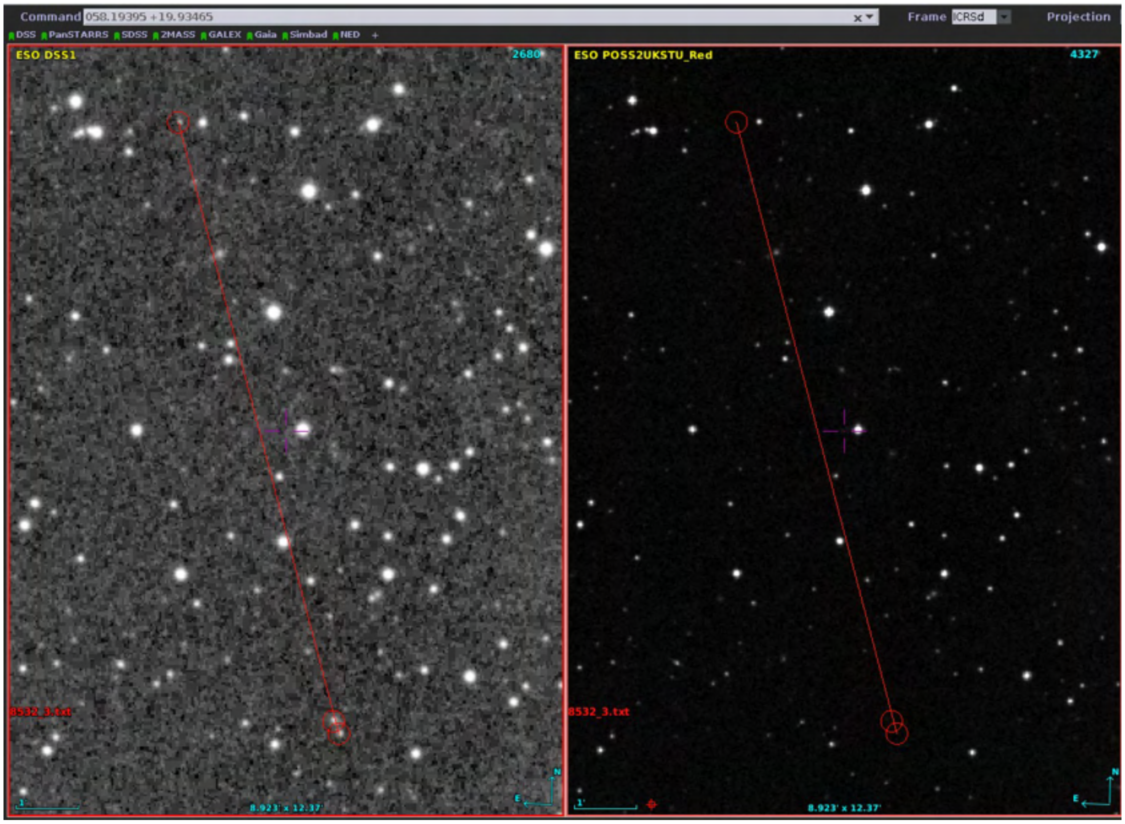


## Figure 72

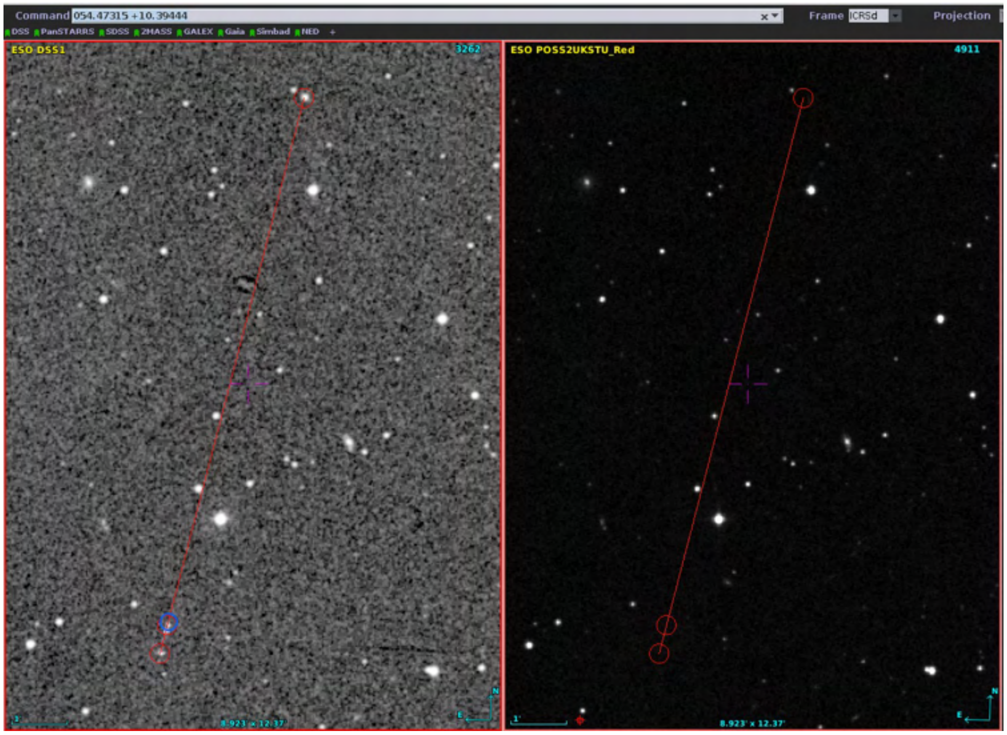


Figure 73

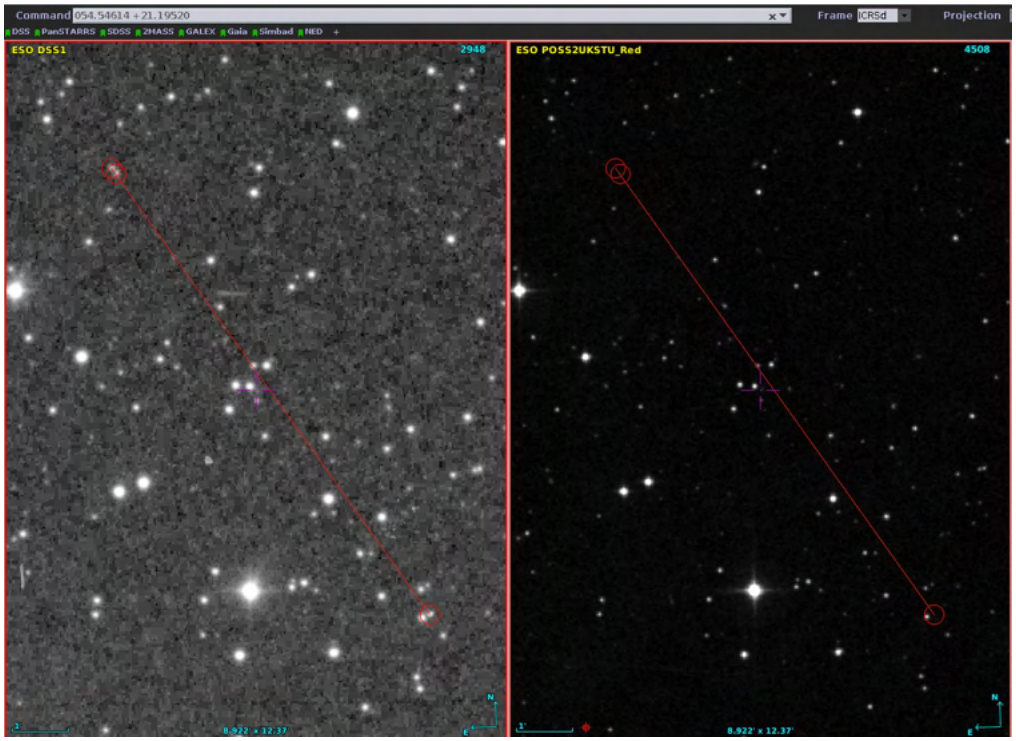


Figure 74

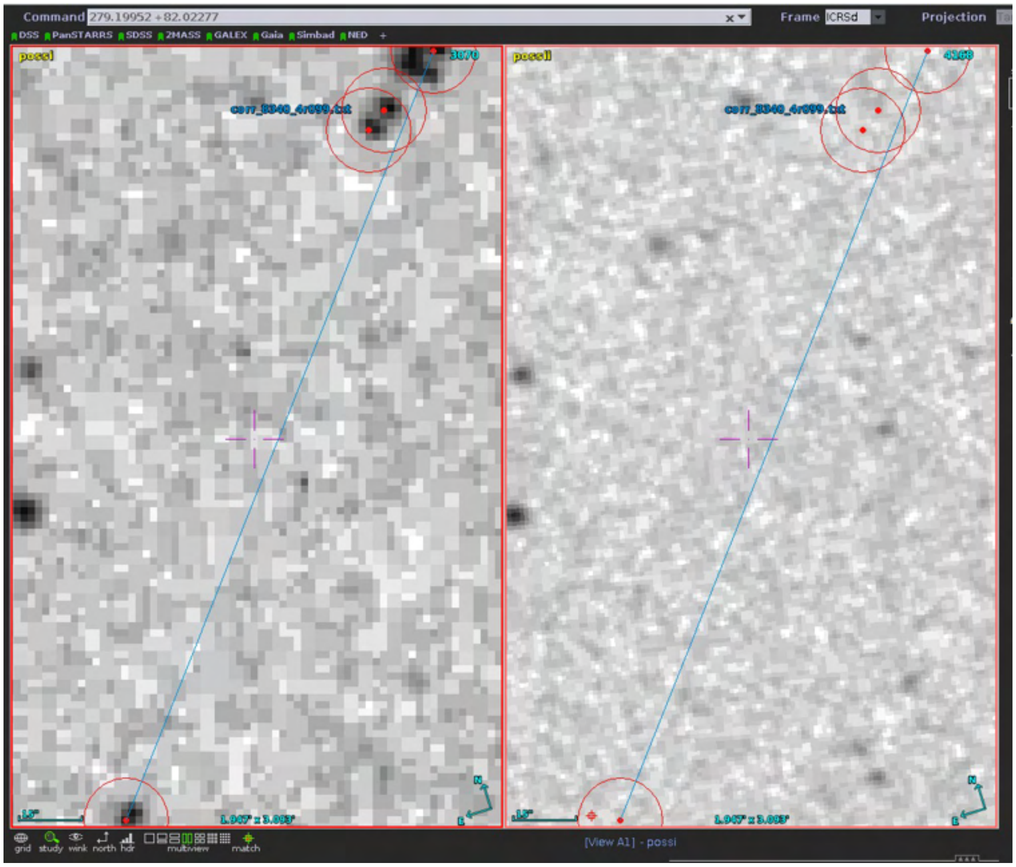


Figure 75

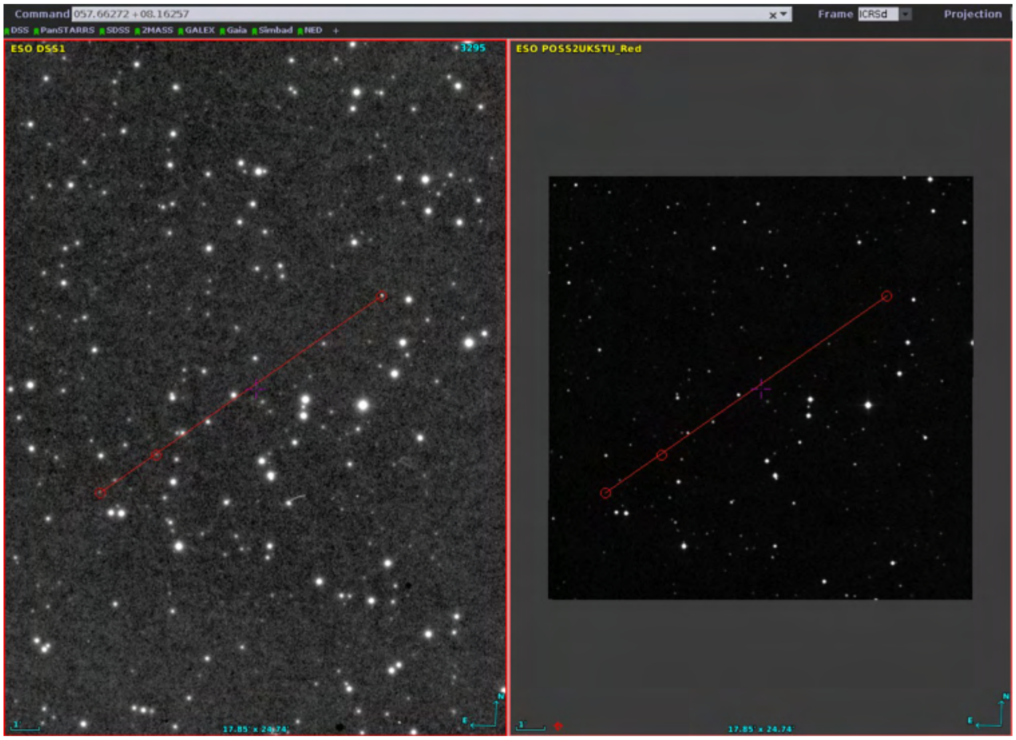


Figure 76

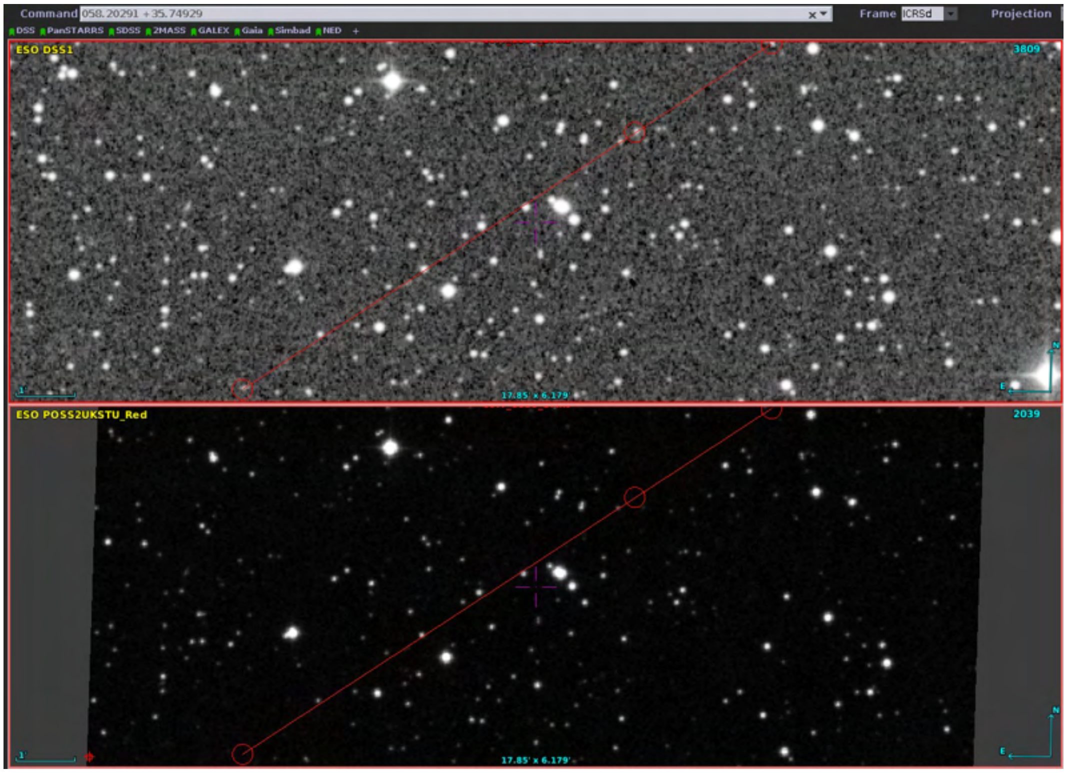


Figure 77

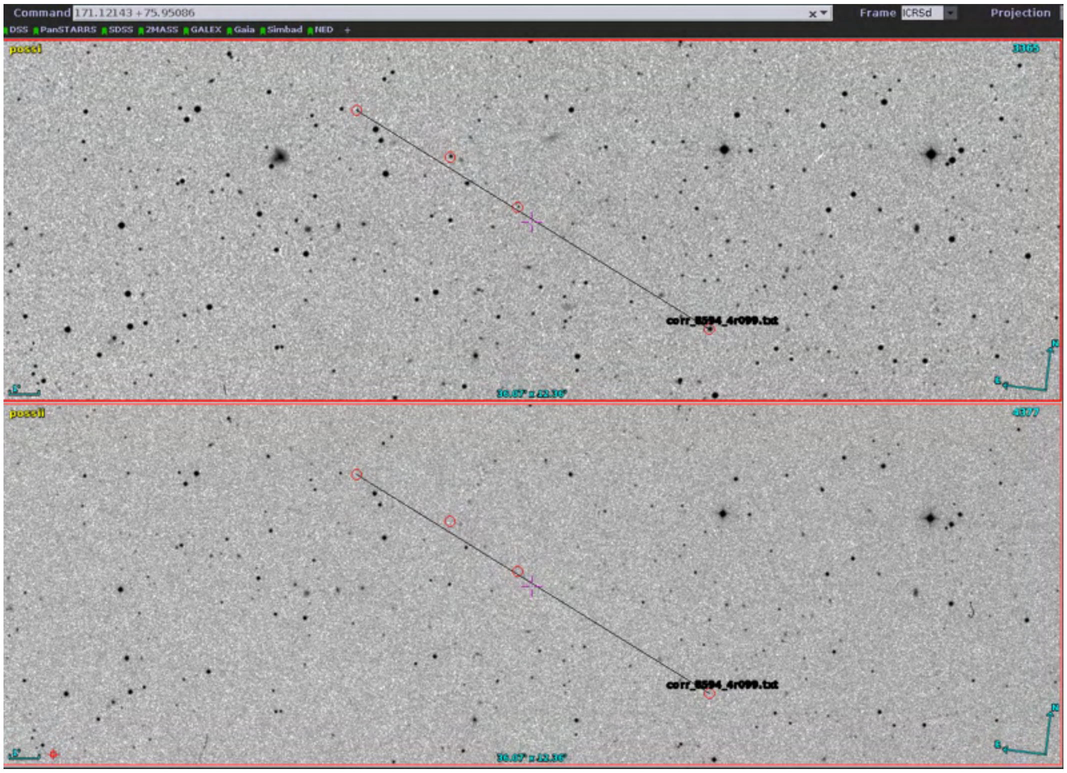


Figure 78

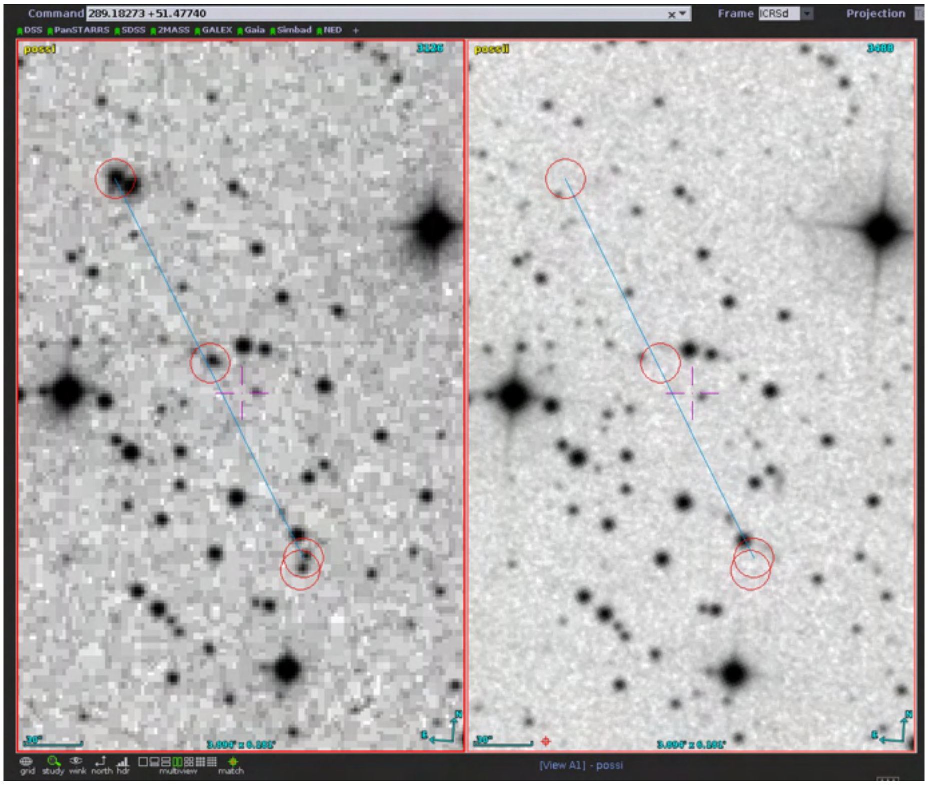


Figure 79

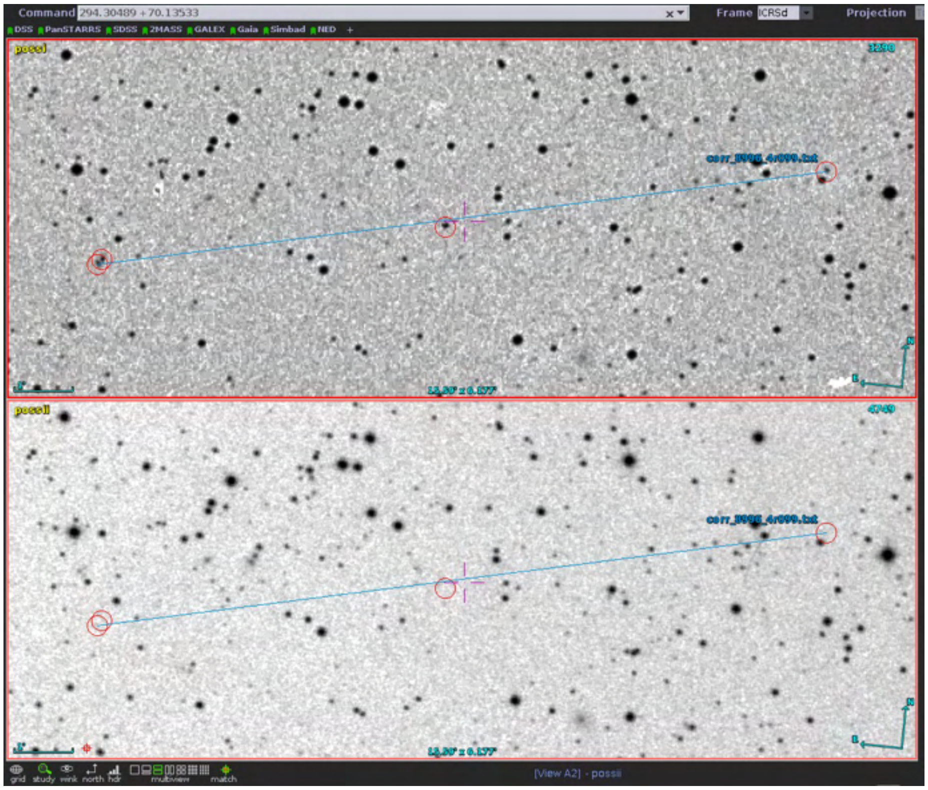


Figure 80

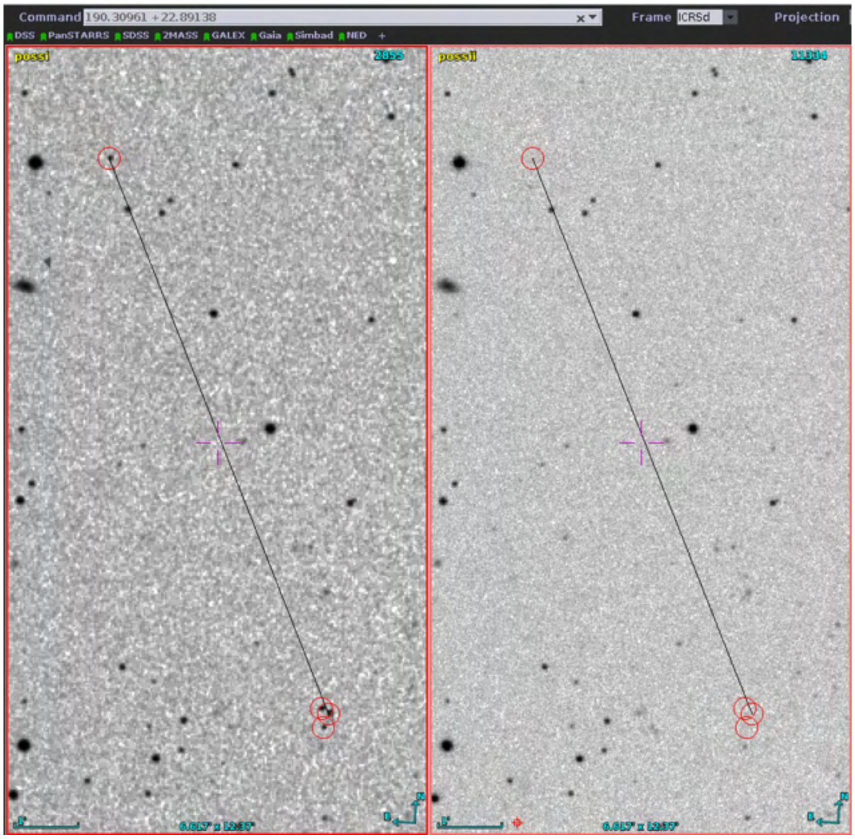


Figure 81

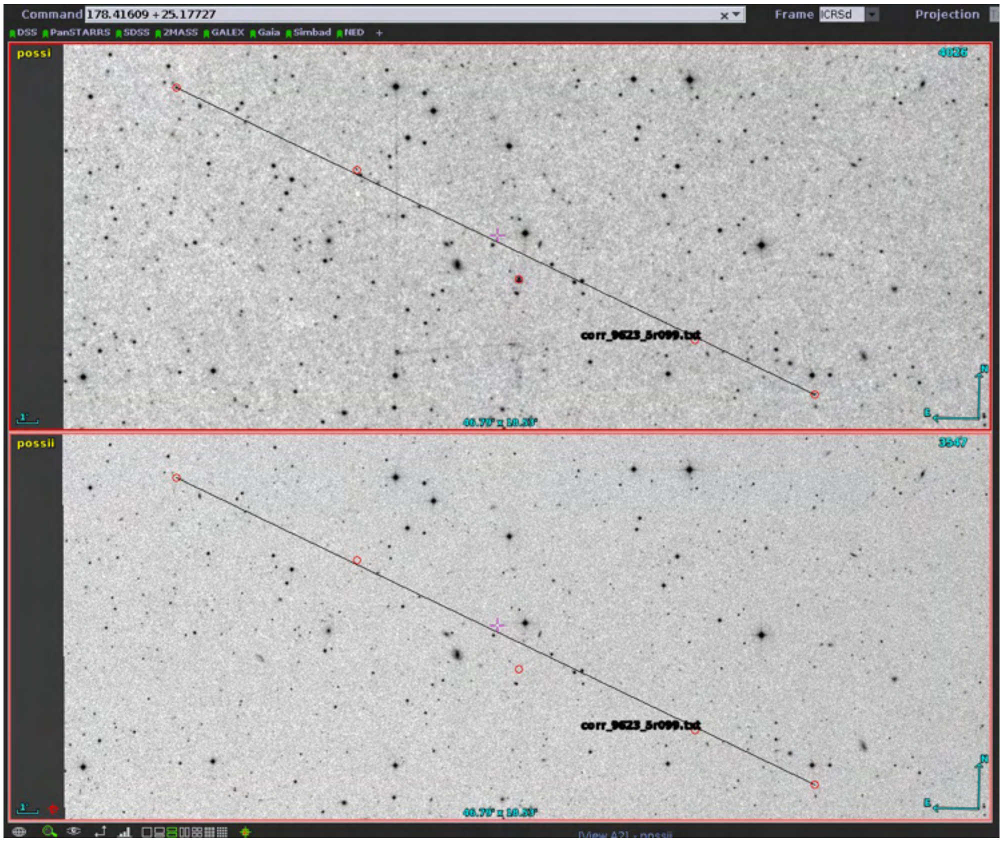


Figure 82

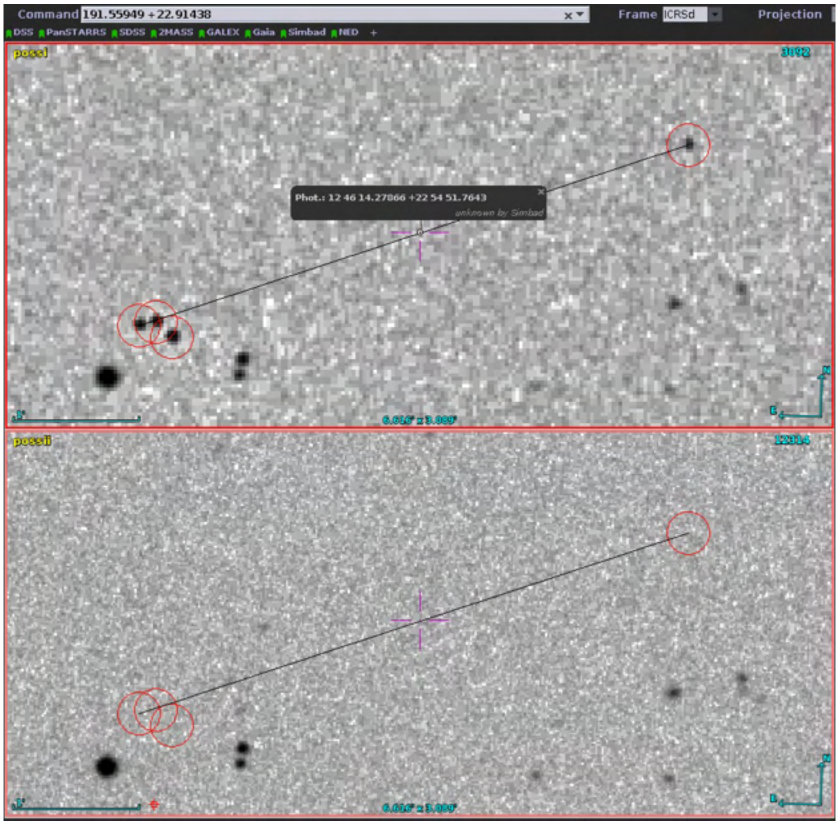


**Figure 83**

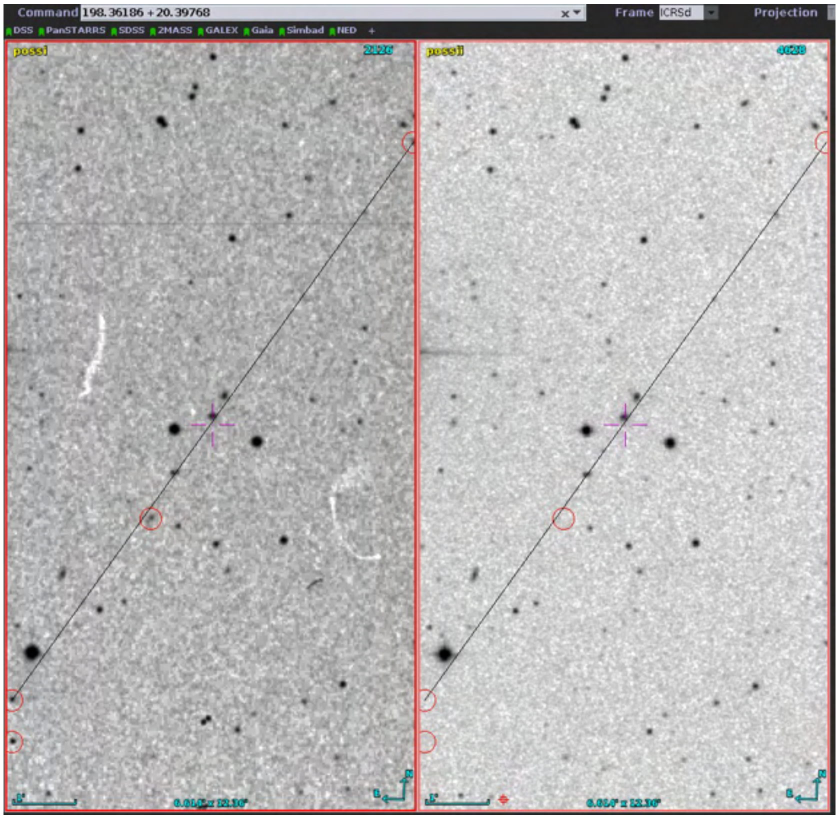


**Figure 84**

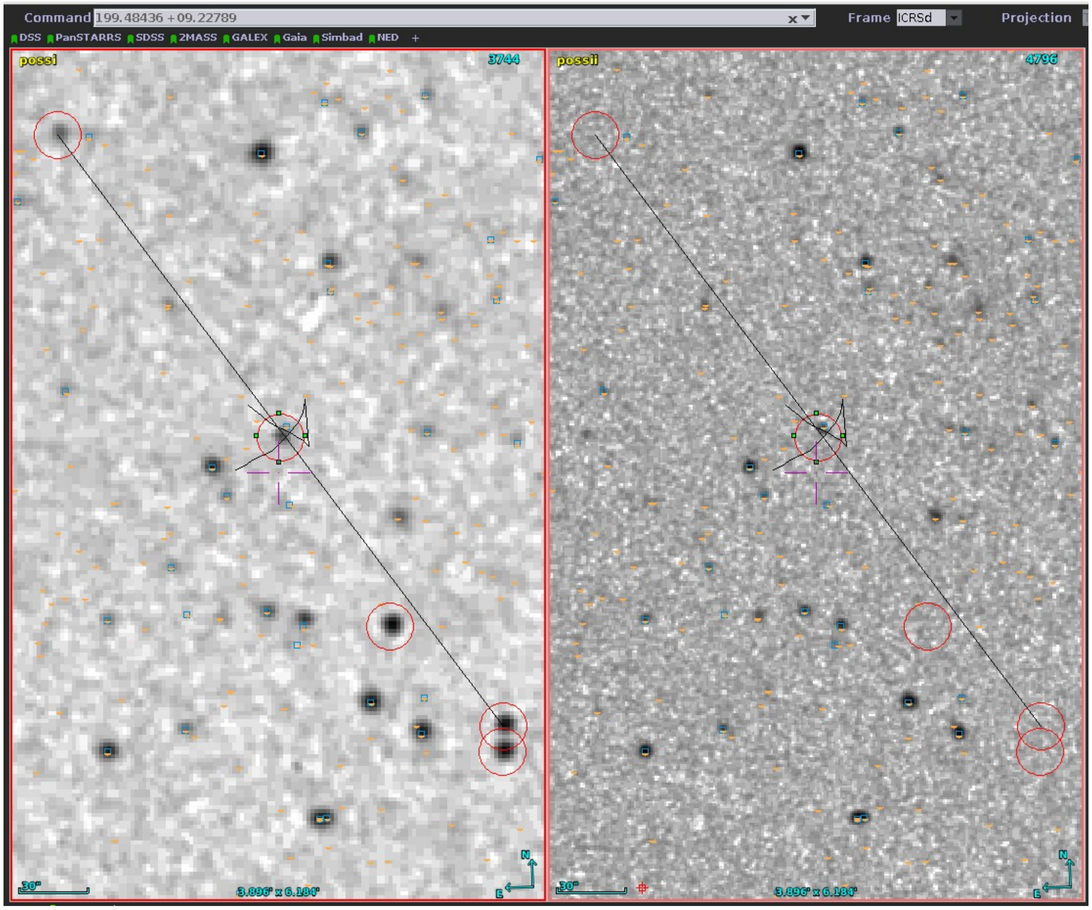

Command 199.48436 +09.22789
Frame ICRSd
Projection
DSS PanSTARRS SDSS 2MASS GALEX Gaia Simbad NED
possi
3744
possii
4796
30"
3.896' x 6.184'
N
E


**Figure 85**
